# Supplementary material for: Quantifying the contributions to diffusion in complex materials
Source: arXiv:2401.06046 source file (2024-03-14)
Supplement: Supplementary file 1 [file supplemental.pdf]

# Quantifying the contributions to diffusion in complex materials: Supplemental material

Soham Chattopadhyay and Dallas R. Trinkle*

*Department of Materials Science and Engineering,*

*University of Illinois, Urbana-Champaign, Illinois 61801, USA*

(Dated: March 7, 2024)

## Abstract

Supplemental material: (1) detailed description of parametrics models and objective function; (2) KMC algorithm and dataset construction; (3) 5-component lattice gas models; (4) high entropy alloy Monte Carlo sampling; (5) cluster expansion and neural network model size optimization; (6) training curves for neural network models; (7) short-range order at 773K; (8) Kinoson densities for Cr, Fe and Mn.

## S1. PARAMETRIC MODELS

Our high entropy alloy states $\chi$ can be mapped onto a vector state by considering a single vacancy, located at the origin, while every other lattice site $\mathbf{x} \neq 0$ has one of five chemical species on it. We describe this with a vector $\mathbf{n}$ where for every lattice site $\mathbf{x} \neq 0$ and species $\alpha$, the value $n_x^\alpha$ is 1 if that site is occupied with species $\alpha$, and 0 otherwise. This simplifies the construction of cluster expansions and permits the implementation of neural network models. The variational principle for mass transport allows us to form parametric approximations for the state positions (also called the "relaxation vectors" [56]) for each species $\alpha$. We can write such approximations as $\mathbf{y}^\alpha(\{\theta\}|\mathbf{n})$, which are vector-valued functions for $\alpha$ in $\mathbf{n}$ with a parameter set $\{\theta\}$. Applying the variational principle, we have

$$2dD^\alpha \geq \min_{\{\theta\}} \sum_{\mathbf{nn'}} p_{\mathbf{n}}^0 W_{\mathbf{n}\to\mathbf{n'}} \left|\delta\mathbf{x}^\alpha(\mathbf{n}\to\mathbf{n'}) + \mathbf{y}^\alpha(\{\theta\}|\mathbf{n'}) - \mathbf{y}^\alpha(\{\theta\}|\mathbf{n})\right|^2, \tag{S1}$$

where $p_{\mathbf{n}}^0$ is the equilibrium Boltzmann probability of state $\mathbf{n}$, and $W_{\mathbf{n}\to\mathbf{n'}}$ is the rate (per unit time) for the system transitioning from state $\mathbf{n}$ to state $\mathbf{n'}$, and $\delta\mathbf{x}^\alpha(\mathbf{n}\to\mathbf{n'})$ is used to denote the displacement of species $\alpha$ during a transition from state $\mathbf{n}$ to state $\mathbf{n'}$.

* dtrinkle@illinois.edu

TABLE S1. Summary of parametric models for $\mathbf{y}^\alpha(\{\theta\}|\mathbf{n})$ for $\alpha$ in $\mathbf{n}$. Scaled bias basis (SBB) and cluster expansion (CE) models involve linear basis expansion of $\mathbf{y}^\alpha(\{\theta\}|\mathbf{n})$ with the corresponding coefficients $\theta^\alpha_\beta$ for SBB and $\theta^\alpha_{\mathbf{v}_c}$ for CE. For the neural network (NN) model, a vector contribution by each atom is predicted as a linear combination of the nearest neighbor directions of the lattice (denoted by $\mathbf{z}$), the coefficients for which are computed using a neural network.

| Prediction Model | Parametric Equation | Optimized Parameters |
|---|---|---|
| Scaled Bias Basis (SBB) | $\mathbf{y}^\alpha(\{\theta^\alpha_\beta\}|\mathbf{n}) = \sum_\beta \theta^\alpha_\beta \sum_{\mathbf{n}''} \Gamma_{\mathbf{n}\to\mathbf{n}''}\delta\mathbf{x}^\beta(\mathbf{n}\to\mathbf{n}'')$ | $\theta^\alpha_\beta$ – expansion coefficient for species $\beta$ |
| Cluster Expansion (CE) | $\mathbf{y}^\alpha(\{\theta^\alpha_{\mathbf{v}_c}\}|\mathbf{n}) = \sum_c a^c(\mathbf{n}) \sum_{\mathbf{v}_c} \theta^\alpha_{\mathbf{v}_c}\mathbf{v}_c$ | $\theta^\alpha_{\mathbf{v}_c}$ – expansion coefficients for symmetrically unique clusters. |
| Neural Network (NN) | $\mathbf{y}^\alpha(\{\theta_{NN}\}|\mathbf{n}) = \sum_{\mathbf{x}:n^\alpha_\mathbf{x}=1} \sum_\mathbf{z} f^{NN}_\mathbf{n}(\{\theta_{NN}\}|\mathbf{x}+\mathbf{z})\mathbf{z}$ <br> $\alpha \neq \text{vac}$ <br> $\mathbf{y}^\text{vac}(\{\theta_{NN}\}|\mathbf{n}) = -\sum_{\alpha\neq\text{vac}} \mathbf{y}^\alpha(\{\theta_{NN}\}|\mathbf{n})$ | $\{\theta_{NN}\}$ – Neural network parameter set. |

As shown in [56], performing kinetic Monte Carlo even just for a single step is variational, and serves as the basis for our computation. The probability matrix to select the next state is $\Gamma_{\mathbf{n}\to\mathbf{n}'} = W_{\mathbf{n}\to\mathbf{n}'}\left(\sum_{\mathbf{n}''} W_{\mathbf{n}\to\mathbf{n}''}\right)^{-1}$, and the mean time in a state is $\tau_\mathbf{n} = \left(\sum_{\mathbf{n}'} W_{\mathbf{n}\to\mathbf{n}'}\right)^{-1}$. We generate a series of sample states using Monte Carlo, then select a single transition; despite using only a single step, we call these "trajectories," and the diffusivity approximation is

$$2dD^\alpha \approx \min_{\{\theta\}} \frac{1}{N_\text{traj}} \sum_{\mathbf{n}\to\mathbf{n}'} \tau_\mathbf{n}^{-1} \left|\delta\mathbf{x}^\alpha(\mathbf{n}\to\mathbf{n}') + \mathbf{y}^\alpha(\{\theta\}|\mathbf{n}') - \mathbf{y}^\alpha(\{\theta\}|\mathbf{n})\right|^2 . \tag{S2}$$

This equation forms the central objective function for all the parametric models used to approximate $D^\alpha$ in this work.

Like traditional machine learning problems, finding the optimal parameters of such models consists of separating the $N_\text{traj}$ samples into training and validation datasets, with the training set used to optimize the parameters and the validation set used to check the generalization of the model. Our objective function is the diffusivity, and involves calculation of two outputs of our ML model: $\mathbf{y}^\alpha(\{\theta\}|\mathbf{n})$ and $\mathbf{y}^\alpha(\{\theta\}|\mathbf{n}')$, from two inputs $\mathbf{n}$ and $\mathbf{n}'$. Also, the diffusivity is a statistical average with a physical meaning as so we use identical sizes of the training and validation sets, in order to keep the scale of statistical errors on both sets similar.

Table S1 summarizes the central governing equations of each type of parametric model used in this work. The are two linear basis models, and one nonlinear model. The "Scaled Bias Basis" (SBB) model[56] is the simplest model that incorporates the jump probabilities. SBB is mathematically simple; however, since the jump probabilities out of both $\mathbf{n}$ and $\mathbf{n}'$ in Equation S2 need to be computed, SBB effectively requires two KMC steps' information. The second linear model is a cluster expansion (CE) model, which approximates the relaxation vectors with a linear combination of vector-valued contributions from clusters of atoms. We count the number of times, $a^c(\mathbf{n})$ that a particular cluster $c$ (which includes all lattice-translated version of it) is observed in the state $\mathbf{n}$. Each time it occurs, it contributes a linear combination of a set of basis vectors $\{\mathbf{v}_c\}$ associated with it.The basis vectors $\mathbf{v}_c$ are constructed in a manner that respects the underlying symmetries of the lattice.

A cluster $c$ is defined as a set of tuples $c = \{(\mathbf{x}_i^c, \alpha_i^c)\}_{i=1,2...\mathrm{b}}$ where $\mathbf{x}_i^c$ denotes the position of the $i^{th}$ lattice site, and $\alpha_i^c$ a particular chemical species. There are as many such $(\mathbf{x}_i^c, \alpha_i^c)$ tuples as the number (b) of atoms we want to consider for a particular cluster (which is called a "b-body" cluster), each representing the occupancy of a particular site by a particular atom; a cluster becomes active in a state $\mathbf{n}$ if all the sites $\mathbf{x}_i^c$ in $\mathbf{n}$ are occupied by the corresponding species $\alpha_i^c$, for $i = 1, 2...\mathrm{b}$. The set of basis vectors vectors $\{\mathbf{v}_c\}$ for the clusters are computed in a process similar to the construction of "vector stars" in [57]

1. Determine all space group operations $\{G\}_c$ for each translationally unique cluster $c$, that leave the sites in $c$ unchanged up to a lattice translation.

2. Construct a set of basis vectors $\{\mathbf{v}_c\}$ that span the space $S_c$, the intersection of the eigenspaces corresponding to an eigenvalue of 1 for the Cartesian rotation matrix of each group operation in $\{G\}_c$. This set of vectors is then assigned to cluster $c$.

The relaxation vector contributions of $c$ are then found as linear combinations of these vectors, as per the equation in Table S1, with coefficients $\theta_{\mathbf{v}_c}$, and implemented for each state $\mathbf{n}$ from the count $a^c(\mathbf{n})$ of occurance of the cluster. As symmetrically related clusters have the same coefficient of linear expansion $\theta_{\mathbf{v}_c}$, the relaxation vectors satisfy the underlying symmetry of the lattice. This cluster expansion is formally identical to the Self-Consistent Mean Field method [18] without the use of closure conditions.

Both linear models can be optimized exactly from simple averages[56]. The relaxation vectors

for some species $\alpha$ are

$$\mathbf{y}_{\mathbf{n}}^{\alpha} = \sum_{i} \theta_i^{\alpha} \mathbf{\Phi}_i(\mathbf{n}) \tag{S3}$$

for basis function $\mathbf{\Phi}_i(\mathbf{n})$ and coefficient $\theta_i^{\alpha}$. Using Equation S1, the optimal values $\theta_i^{*,\alpha}$ are

$$\theta_i^{*,\alpha} = \sum_{j} \overline{W}_{ij}^{\dagger} \overline{b}_j^{\alpha} \tag{S4}$$

where † denotes a pseudo-inverse. The elements of the matrix $\overline{\mathbf{W}}$ are

$$\overline{W}_{ij} = -\frac{1}{2} \sum_{\mathbf{n},\mathbf{n}'} p_{\mathbf{n}}^{0} \Gamma_{\mathbf{n}\to\mathbf{n}'} \tau_{\mathbf{n}}^{-1} \Delta\mathbf{\Phi}_i(\mathbf{n} \to \mathbf{n}') \cdot \Delta\mathbf{\Phi}_j(\mathbf{n} \to \mathbf{n}') \tag{S5}$$

where $\Delta\mathbf{\Phi}_i(\mathbf{n} \to \mathbf{n}') = \mathbf{\Phi}_i(\mathbf{n}') - \mathbf{\Phi}_i(\mathbf{n})$. The elements $\overline{b}_i$ are

$$\overline{b}_i^{\alpha} = -\frac{1}{2} \sum_{\mathbf{n},\mathbf{n}'} p_{\mathbf{n}}^{0} \Gamma_{\mathbf{n}\to\mathbf{n}'} \tau_{\mathbf{n}}^{-1} \delta\mathbf{x}^{\alpha}(\mathbf{n} \to \mathbf{n}') \cdot \Delta\mathbf{\Phi}_i(\mathbf{n} \to \mathbf{n}') \tag{S6}$$

We optimize the parameters the training set of single-step KMC samples, and validate with our validation set.

The third parametric model is a neural network (NN) model. Here, for an atomic (non-vacancy) species $\alpha$, the relaxation vectors are written as a sum of vectors contributed by individual $\alpha$ atoms in $\mathbf{n}$. We use linear combinations of the nearest neighbor directions of the lattice (denoted by $\mathbf{z}$ in Table S1) to find these contributions. The coefficients of such linear combinations, $f_{\mathbf{n}}^{NN}(\{\theta_{NN}\}|\mathbf{x})$ in Table S1 are computed using a neural network. Our neural network layers follow the convolutional design in [34], which respects the underlying rotational symmetries of the lattice. In this network design, for a particular state $\mathbf{n}$, the successive mathematical operations to accept a representation $I_l^{\mathbf{n}}$ of the state as the input to the $l^{\text{th}}$ network layer, and return $I_{l+1}^{\mathbf{n}}$ as the output (input to the $(l+1)^{\text{th}}$ network layer) involves a linear convolution operation followed by a non-linear transformation. This process can be written mathematically as

$$F_l^{\mathbf{n}}(o, g, \mathbf{x}) = \sum_{i,\mathbf{r}} I_l^{\mathbf{n}}(i, \mathbf{x} + \mathbf{r}) \Psi_l(o, i, g^{-1}\mathbf{r}) + b_l(o) \tag{S7}$$

$$I_{l+1}^{\mathbf{n}}(o, \mathbf{x}) = \frac{1}{N_g} \sum_{g} \kappa(F_l^{\mathbf{n}}(o, g, \mathbf{x})) \tag{S8}$$

In these equations, $i$ and $o$ represent input and output channels respectively, $g$ represents a symmetry operation, $N_g$ is the total number of symmetry operations in the crystal's space group, and $\mathbf{r}$ runs over nearest neighbor directions, as well as the $\mathbf{0}$ vector. $\Psi_l(o, i, \mathbf{r})$ are the convolutional filter elements, $b_l(o)$ is a bias term assigned to output channel $o$, and $\kappa$ is a non-linear function, which we chose to be the widely used "Softplus" function given as $\kappa(x) = \log(1 + e^x)$ [58]. All the filter elements (elements of $\Psi$) for every layer and the bias elements constitute the trainable parameter set of the network, represented as the set $\{\theta_{NN}\}$ in Table S1. As discussed in [34], these operations ensure that if the input to a layer is transformed by some symmetry operation, the output automatically transforms by the same.

The input for the very first layer of the neural network, identified with $l = 0$, is constructed to have as many channels as the number of species, such that

$$I_0^{\mathbf{n}}(\alpha, \mathbf{x}) = n_{\mathbf{x}}^{\alpha} \tag{S9}$$

The last layer of the neural network is made to produce a single channel representation of $\mathbf{n}$ given by:

$$F_{\text{Last}}^{\mathbf{n}}(g, \mathbf{x}) = \sum_{i,\mathbf{r}} I_{\text{Last}}^{\mathbf{n}}(i, \mathbf{x} + \mathbf{r})\Psi_{\text{Last}}(i, g^{-1}\mathbf{r}) + b_{\text{Last}} \tag{S10}$$

$$f_{\mathbf{n}}^{NN}(\{\theta_{NN}\}|\mathbf{x}) = \frac{1}{N_g}\sum_{g} \kappa(F_{\text{Last}}^{\mathbf{n}}(g, \mathbf{x})) \tag{S11}$$

For some species $\alpha$ that is not the vacancy, these output representations are then used as coefficients to linearly combine the nearest neighbor vectors ($\mathbf{z}$) to produce the relaxation vector approximations as:

$$\mathbf{y}^{\alpha}(\{\theta_{NN}\}|\mathbf{n}) = \sum_{\mathbf{x}:n_{\mathbf{x}}^{\alpha}=1} \sum_{\mathbf{z}} f_{\mathbf{n}}^{NN}(\{\theta_{NN}\}|\mathbf{x} + \mathbf{z})\mathbf{z} \tag{S12}$$

All neural networks in this work were implemented using the PyTorch package [59] for automatic differentiation and trained with the Adam gradient descent algorithm [60] with Equation S2 as the objective function, with a step size of $10^{-3}$ and a batch size of 128.

CE and NN models predict relaxation vectors from purely configurational information. Therefore, both of these models require the rate information from one state, while SBB requires the rate information for two states. We can also combine such models with the SBB model with two states of rate information; this is the scaled residual bias correction[56], where the residual bias after

optimization is used to make a further improvement in the diffusivity. The optimal neural network prediction of the relaxation vector of species $\alpha$ as $\mathbf{y}^{\alpha}(\{\theta^{*}_{NN}\}|\mathbf{n})$, the relaxatuion

$$\begin{aligned}
\mathbf{y}^{\alpha}(\{\theta^{*}_{NN}, \theta^{\alpha}_{\beta}\}|\mathbf{n}) = &\mathbf{y}^{\alpha}(\{\theta^{*}_{NN}\}|\mathbf{n}) \\
&+\theta^{\alpha}_{\alpha}\sum_{\mathbf{n}''}\Gamma_{\mathbf{n}\to\mathbf{n}''}\left[\delta\mathbf{x}^{\alpha}(\mathbf{n}\to\mathbf{n}'') + \mathbf{y}^{\alpha}(\{\theta^{*}_{NN}\}|\mathbf{n}'') - \mathbf{y}^{\alpha}(\{\theta^{*}_{NN}\}|\mathbf{n})\right] \\
&+\sum_{\beta\neq\alpha}\theta^{\alpha}_{\beta}\sum_{\mathbf{n}''}\Gamma_{\mathbf{n}\to\mathbf{n}''}\delta\mathbf{x}^{\beta}(\mathbf{n}\to\mathbf{n}'')
\end{aligned} \tag{S13}$$

and use Equation S2 to optimize just the parameters $\theta^{\alpha}_{\alpha}$ and $\theta^{\alpha}_{\beta}$. This final equation is our accurate "NN+SRBC" calculation.

## S2. KINETIC MONTE CARLO SIMULATION

In order to compute our empirical objective function Equation S2 and optimize our parametric models, we need to simulate single step KMC trajectories. In order to then assess the quality of the diffusivity predictions by such optimal parametric models, we also perform full KMC simulations of several steps to get a "ground truth" estimate of the diffusivity. Each such KMC step is carried out using a "mean residence time" algorithm, similar to [61], and consistent with Equation S2, described in Algorithm 1.

The computation of the diffusivity traces $D^{\alpha}$ then involves computing mean of squared displacements divided by time for multiple trajectories with desired number of steps as described in Algorithm 2. In all our calculations, the attempt frequencies are assumed same and constant for all atomic species.

**Algorithm 1:** Pseudo-code to perform a single KMC step as used in this work, and return the displacement of a desired species $\alpha$. Note that the rates are computed in units of the attempt frequency $\nu^0$, and the time of the step in units of $(\nu^0)^{-1}$.

**input :** $\mathbf{n}$ Initial state for the KMC step.
**input :** $k_B$, $T$ : Boltzmann constant and temperature respectively.
**input :** $\delta\mathbf{x}_{nn}$ : Array of shape ($z \times 3$), the nearest neighbor vacancy jump vectors, $z$ being the coordination number.
**output:** $\delta\mathbf{x}^\alpha$: The displacement of species $\alpha$.
**output:** $\tau_\mathbf{n}$: Mean residence time in state $\mathbf{n}$, the time for the KMC step.

Initialize $W, P, C$: Each an array of $z$ zeroes.
Initialize $r = 0$ , The total escape rate out of $\mathbf{n}$
Compute vacancy jump barriers $E_b^j$ for all $j = 1, 2, ...z$ vacancy jumps out of $\mathbf{n}$.
Compute rates $W[j] = \mathrm{e}^{-E_b^j/(k_BT)}$ for all $j = 1, 2, ...z$
$r = \mathrm{sum}(W[j]$ for all $j = 1, 2, ...z)$
$\tau_\mathbf{n} = 1/r$
$P[j] = W[j]/r$ for all $j = 1, 2, ...z$
$C[j] = \mathrm{sum}(P[k]$ for all $k = 1, 2, ...j)$ for all $j = 1, 2, ...z$
get random number $q \sim \mathcal{U}(0, 1)$
get integer $s \geq 1$ such that $C[s-1] < q \leq C[s]$ with $C[0] = 0$
set vacancy displacement $\delta\mathbf{x}^{\mathrm{vac}} = \delta\mathbf{x}_{nn}[s]$
set displacement $\delta\mathbf{x}^\beta = -\delta\mathbf{x}_{nn}[s]$ for species $\beta$ occupying the $s^{\mathrm{th}}$ vacancy nearest neighbor site, $\mathbf{0}$ for all other species
Exchange vacancy and $\beta$ positions in state $\mathbf{n}$
**return** $\tau_\mathbf{n}$, $\delta\mathbf{x}^\alpha$ for all species $\alpha$

**Algorithm 2:** Pseudo-code for the computing desired number of KMC steps and diffusivities $D^\alpha$ for a desired species $\alpha$ using Algorithm 1.

```
input  : N_traj, N_step : No. trajectories and KMC steps per trajectory respectively.
input  : n_i, i = 0, 1, 2..., N_traj: Initial states for each trajectory drawn from Boltzmann
         distribution.
input  : k_B, T : Boltzmann constant and temperature respectively.
input  : δx_nn : Array of shape (z × 3), the vacancy jump vectors, z being the coordination
         number.
output: D^α: The diffusivity of species α, in units of V_0 k_B T, V_0 being the total system
         volume.
set L^{α,α} = 0
foreach i in (1, 2..., N_traj) do
    set R^α = 0
    set t_traj = 0                                   // The total time.
    foreach step in (1, 2..., N_step) do
        get (τ_{n_i}, δx^α) for species α using Algorithm 1 with input as state n_i (updated after
         each step in Algorithm 1)
        R^α += δx^α
        t_traj += τ_{n_i}
    end
    D^α += ν^0 |R^α|^2 / (6 t_traj)                  // ν^0:  the attempt frequency
end
return D^α / N_traj
```

## S3. VACANCY DIFFUSION SIMULATION IN MODEL LATTICE GAS SYSTEMS

### A. 5-Component Lattice Gas

Changing the rates for our system allows us to better understand the performance of different models: the “Random” and “Ordered” rate systems in our main paper, which differ in the way the vacancy jump barriers and rates are computed as a function of the atomic configurations in a state. In all such simulations, the states consist of atomic species distributed on 511 atomic sites and a single vacancy site in $8 \times 8 \times 8$ primitive FCC supercells under periodic boundary conditions. The energy of every state is identical, only exchange rates change.

Figure S5 shows that the exchange barriers in our high entropy alloy are well-described by a normal distribution. Each atomic species $\alpha$ has a mean barrier $\mu_b^\alpha$ with standard deviation $\sigma_b^\alpha$ for vacancy-$\alpha$ atom exchange. We then distribute these migration barriers $E_b^\alpha$ accordingly, and the jump rates are

$$\nu_\alpha = \nu^0 \exp\left(-\frac{E_b^\alpha}{k_B T}\right) \tag{S14}$$

with attempt frequency $\nu^0$ (constant for all species). The migration barriers $E_b^\alpha$ were computed using a pseudo-random number generator (PRNG) based on the atomic occupancies within the third nearest neighborhood of the vacancy in both the initial and final states of a vacancy-atom exchange for the “Random” rate simulations. Steps were taken to ensure that the rates so obtained are single-valued and satisfy symmetry and detailed balance. The algorithm to obtain these rates $\nu_\alpha$ in these simulations is shown in Algorithm 3. Similar simulations of high-entropy alloys with randomly generated jump rates were also done elsewhere recently [48–50], although without preserving the crystal’s symmetry and/or without maintaining detailed balance.

For the “Ordered” rate simulations, the dependence of the jump rates on configurations was limited to only which atom executes an exchange jump with the vacancy. This was done by fixing the vacancy exchange rate of each atomic species to the average rate $\overline{\nu_\alpha} = \nu^0 \exp\left[-\frac{\mu_b^\alpha}{k_B T} + \frac{1}{2}\left(\frac{\sigma_b^\alpha}{k_B T}\right)^2\right]$, irrespective of the surrounding neighborhood configuration. This makes the jump probabilities only a function of the first nearest neighborhood of the vacancy, and also provides a much simpler rate landscape than the “Random” rate systems. Systems with such fixed jump rates of the atomic species have also been studied elsewhere in the literature [57, 62, 63].

With these methods to compute the jump rates for the “Ordered” and “Random” rate systems, we performed one KMC step from 20000 starting states with randomly assigned atomic occu-

**Algorithm 3:** Pseudo-code for computing jump rates in the "Random" rate systems. The returned jump rates are in units of the attempt frequency. Note that the vacancy is assumed to occupy the $0^{th}$ site in all states.

**input :** $\mathbf{n}, \mathbf{n}'$ : Initial, final states of vacancy jump
**input :** species $\alpha$ : The species exchanging positions with the vacancy
**input :** $\mathrm{v}_{nn}$ : nearest neighbor shell around the vacancy site we consider site occupancies up to. The sites are visited in ascending order of their indices.
**output:** The jump rate $W_{\mathbf{n}\to\mathbf{n}'}$

**Function** `SeedState`($\mathbf{n}''$):
    $s_{\mathbf{n}''} = 0$
    **foreach** *group operation* $g \in$ *the space group* $G$, **do**
        $\mathbf{n}''_{\mathbf{g}} = g\mathbf{n}''$    `// transform the state symmetrically.`
        $s_g = 0$
        $c = 1$
        **foreach** *site* $i(\geq 1) \in \mathrm{v}_{nn}$ **do**
            $s_p \longleftarrow$ Integer label of species at site $i$ in state $\mathbf{n}''_{\mathbf{g}}$
            $s_g += (c * 10000) * 2^{s_p}$
            $c += 1$
        **end**
        $s''_{\mathbf{n}} += s_g$
    **end**
    **return** $s''_{\mathbf{n}}$
**End Function**
$s_{\mathbf{n}} =$ `SeedState`($\mathbf{n}$)
$s_{\mathbf{n}'} =$ `SeedState`($\mathbf{n}'$)
$s_{\mathbf{n}\to\mathbf{n}'} = \lfloor \frac{s_{\mathbf{n}} s_{\mathbf{n}'}}{s_{\mathbf{n}} + s_{\mathbf{n}'}} \rfloor$
Seed pseudo-random number generator $\mathcal{N}\left(\frac{\mu_b^\alpha}{k_B T}, \frac{\sigma_b^\alpha}{k_B T}\right)$ with $s_{\mathbf{n}\to\mathbf{n}'}$
Draw barrier $E_b^\alpha(T) \sim \mathcal{N}\left(\frac{\mu_b^\alpha}{k_B T}, \frac{\sigma_b^\alpha}{k_B T}\right)$
**return** $\mathrm{e}^{-E_b^\alpha(T)}$

pancies on the lattice sites, with desired compositions, to construct datasets of pairs of initial ($\mathbf{n}$) and final ($\mathbf{n}'$) states of single KMC steps using the KMC algorithm described in Section S2. The vacancy-atom exchange rates out of the final states $\mathbf{n}'$ were also computed for use with the SBB model. These single step samples were then split equally into training and validation sets. We then optimized, via Equation S2, our parametric SBB, CE and NN models to compute the diffusivities, $D^{\text{fast}}$, of the "fast" species, which has the largest $\overline{\nu_\alpha}$ (with all other species designated as "slow" species).

In both the "Random" and "Ordered" systems, the composition of the system was fixed to $\approx 20\%$ by allowing a maximum of 103 and minimum 102 atoms of any given species in any state, and datasets were constructed at temperatures of 1073 K, 1173 K, 1273 K and 1373 K. The

distributions of the migration barriers for the 5 species in the CR-5 system are summarized in Figure S1, with the histograms denoting the distribution obtained from our "Random" rate dataset at 1073 K using Algorithm 3 shown as an example.

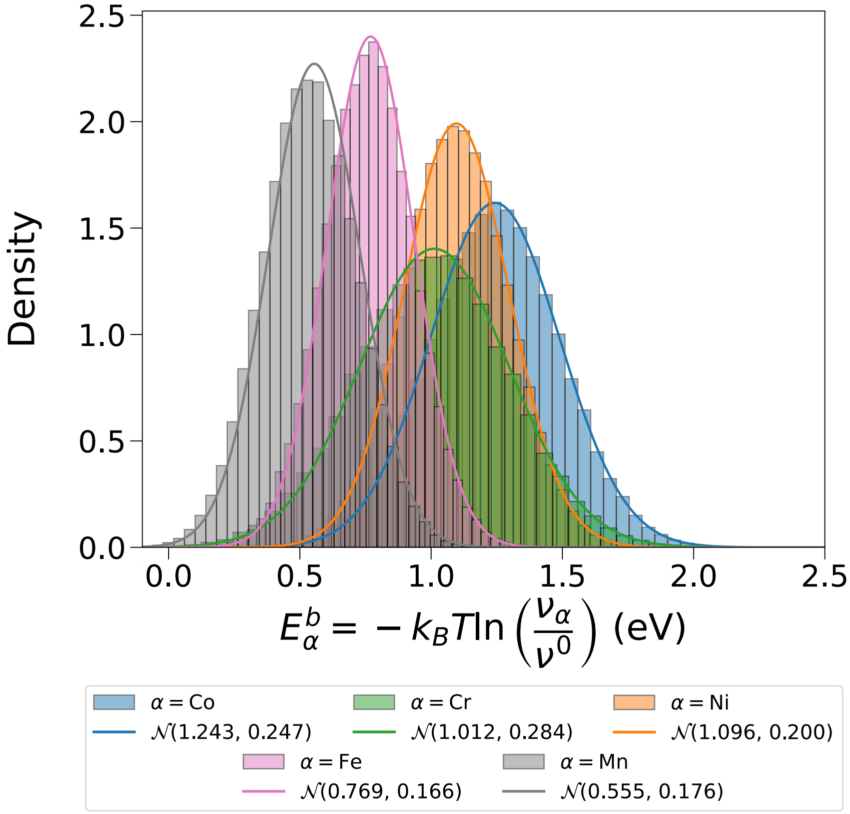


FIG. S1. Distributions used for the species exchange barriers in the "Random" rate system. The migration barriers for each species $\alpha$ (= Co, Ni, Cr, Fe, Mn) are taken to follow normal distributions $\mathcal{N}(\mu_b^\alpha, \sigma_b^\alpha)$, shown with solid lines with the values of the mean $\mu_b^\alpha$ and standard deviation $\sigma_b^\alpha$ shown for each species. These quantities were estimated from the sample means and standard deviations of vacancy jump barriers simulated using the MEAM potential in [47]. The histograms correspond to statistics obtained from the 1073 K single KMC step data set using Algorithm 3, provided as an example of actual obtained rate distributions in our "Random" rate simulations. The rates $\nu_\alpha$ are in units of the attempt frequency $\nu^0$, which is assumed constant and fixed for all the species.

At each temperature, full KMC simulations were also performed up to 1000 steps for both the "Random" and "Ordered" rate systems, and the diffusivities of the "fast" species were averaged over 10000 such independent KMC trajectories.

### B. 2-Component Lattice Gas

A binary lattice gas system, was also tested similar to the 5-component lattice gases in the previous section. The two atomic species in the binary systems are labelled the "fast" and "slow" species respectively, while concentration is varied. The "Random" rates come from a log-normal distribution with means $\overline{\nu_{\text{fast}}} = 1.0$ and $\overline{\nu_{\text{slow}}} = 10^{-3}$ and standard deviations of 2.0. We also chose $\text{v}_{nn} = 5$ in Algorithm 3 to get a good distribution of the barriers. For the "Ordered" rate case, $\overline{\nu_{\text{fast}}} = 1.0$ and $\overline{\nu_{\text{slow}}} = 10^{-3}$.

Figure S2 shows the binary case as a function of composition. We see that the 2-component "Ordered" rate system exhibits the well known percolation phenomenon [56, 63, 64], where, if $\overline{\nu_{\text{fast}}} \gg \overline{\nu_{\text{slow}}}$, then as $c_{\text{slow}}$ increases, $D^{\text{fast}}$ decays toward zero due to increasingly correlated vacancy-"fast" atom exchanges. We also find that the "Random" rate system exhibits more correlation than the "Ordered" case due to faster rates being accessible to the "fast" species. This behavior is also analogous to the 5-component lattice gas systems. As in tge 5-component case, the "Ordered" rate system, the NN models can predict transport coefficients as accurate as 100-1000 steps of KMC from a single KMC step, followed by the CE model, and the SBB models show the worst disagreement with KMC results. Conversely, for the 2-component "Random" rate systems also the SBB models show better agreement with KMC results than both the NN and CE models, which are now generally quite poor predictors of the diffusivity.

We note Figure S2, however, that as $c_{\text{slow}}$ becomes higher, the NN and CE models become able to predict better transport coefficients for the 2-component . This may be because as $c_{\text{slow}}$ increases, the atomic neighborhood around the vacancy starts to become less and less unique. For example, let us consider occupancies of sites within the second nearest neighborhood of the vacancy in the starting states of the single KMC steps in our 2-component "Random" rate datasets. Then, among the 10000 samples in the validation set at $c_{\text{slow}} = 85\%$, 2185 samples were found that had different configurations compared to those in training set, despite the states being constructed randomly. For reference, at $c_{\text{slow}} = 60\%$, this number was 9299 samples. This is coupled with the fact that correlations between atomic jumps can become more spatially local around the vacancy due to increased back-and-forth exchanges between increasingly isolated vacancy-fast atom pairs as $c_{\text{slow}}$ increases. This allows the NN and CE models to more easily learn the effects of such local environments on the diffusivity of the "fast" atom.

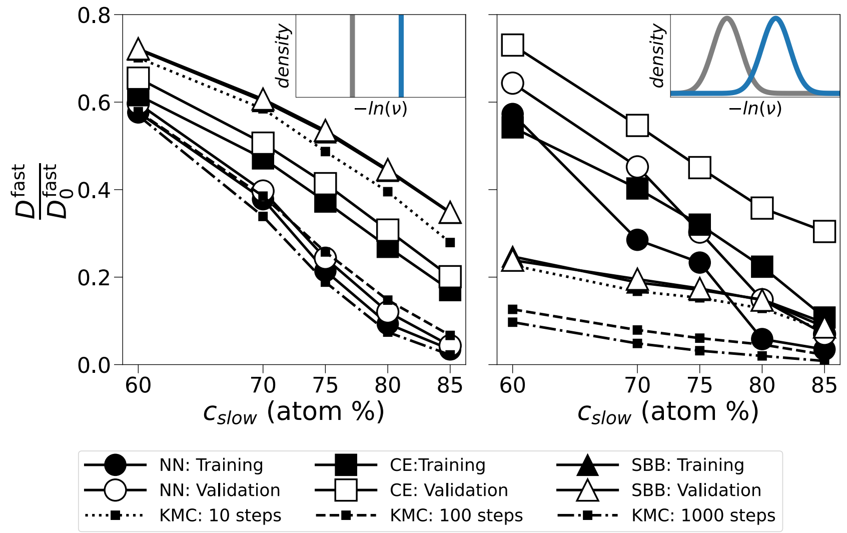


FIG. S2. Comparison of the performance of optimal parametric models for 2-component "Ordered" (left) and "Random" (right) rate systems in predicting the diffusivity $D^{\text{fast}}$ of the "fast" species. The "Ordered" rate system shows the percolation phenomenon, with $D^{\text{fast}}$ decreasing as $c_{\text{slow}}$ increases due to increased correlation in vacancy-"fast" atom diffusion. Such correlations are more pronounced in the "Random" rate case due to faster rates available for the "fast" species. The model performance shows the same trend as the 5-component lattice gases in Figure 1 of our main paper, with the neural network model being the best predictor in the "Ordered" rate systems, and the SBB model in the "Random" rate systems.

## S4. VACANCY DIFFUSION SIMULATION IN AN INTERACTING HIGH-ENTROPY ALLOY

To simulate diffusion in a "Complex" rate system, we also consider 5-component Co-Ni-Cr-Fe-Mn high-entropy alloys with the rates computed using Equation S14, but with the migration barrier of every vacancy-atom exchange jump computed using the actual MEAM potential in [47] simulated at 1073 K, 1173 K, 1273 K and 1373 K, at which the alloy has been shown to be nearly random [47] although with some ordering [48]. We used 5×5×5 orthogonal FCC supercells with 499 atomic sites and one vacancy site with a lattice parameter of 3.595 Å, the equilibrium lattice constant[47]. These cells have one species with 99 atoms, and all other four have 100 atoms. We use Metropolis Monte Carlo to generate initial states, then nudged elastic band to calculate energy barriers for the vacancy to jump. We also perform kinetic Monte Carlo simulations of longer trajectories to determine the converged diffusivity.

We performa a standard Metropolis Monte Carlo (MC) sampling at constant NVT[65] using the MEAM potential in [47] to compute state energies. With the vacancy site fixed at the origin and the atoms at on-lattice positions, each MC step then consists of swapping two randomly selected sites occupied by different atomic species. Swaps are accepted with probability $\exp\left(\frac{-\delta E}{k_B T}\right)$, where

$\delta E$ is the change in the energy of the system after a swap; the energies correspond to the relaxed configurations with a Conjugate Gradient method as implemented in the LAMMPS software [66] with a maximum force tolerance per atom of $10^{-3}$ eV/Å and with a constant supercell volume. 200 different such MC runs were carried out at each temperature, each starting from a randomly initialized (nominally equicomposition) state. The resulting convergence plot of the energies is shown in Figure S3. It is seen that by 10000 steps, reasonable convergence is achieved in the state energies. States were then gathered from the $10000^{th}$ step onward, at intervals of 1000 steps, until 100 states from each of the 200 simulations were obtained, for a total of 20000 states, at each temperature. These states were the initial states to construct single KMC step datasets for diffusivity prediction using Equation S2. These were then divided equally to form our training and validation sets using single KMC steps, and it was ensured that states from the same Monte Carlo simulation are initially present only in either of the two sets to maintain disjointedness between training and validation samples.

To assess the independence of the states gathered during the MC simulations, we examine the autocorrelation[67] of the state energies,

$$C_E(t) = \frac{1}{N-t} \sum_{i=1}^{N-t} \frac{(E(i) - \langle E \rangle)(E(i+t) - \langle E \rangle)}{\sigma_E^2} \tag{S15}$$

where $E(i)$ corresponds to the energy of the $i^{\text{th}}$ state gathered from a MC run, and $E(i+t)$ to that out of the next $t^{th}$ state gathered in the same run. $\langle E \rangle$ and $\sigma_E^2$ correspond to the mean and standard deviations, respectively, of the energies of all the states gathered from a given MC run. $C_E(t)$ measures the statistical correlation between states gathered at intervals of $t$ states.Figure S4 shows $C_E(t)$ averaged across the 200 different MC simulations at each temperature. The autocorrelation is small after a lag of 1, indicating that each state is sufficiently uncorrelated from the one gathered after it, and all auto-correlations quickly decay towards zero, indicating sufficient statistical independence of all the states. We observe that as the temperature increases, The lag of 1 corresponds to 1000 MC swaps, at which interval the states were gathered from each independent MC simulation (with 100 states gathered from each).

Once the initial states **n** in Equation S2 were gathered from the MC simulations, NEB [68] calculations were carried out using LAMMPS, with 11 images including the initial and final atomic configurations for each of the 12 nearest-neighbor vacancy-atom exchange jumps out of each state. For these calculations, the atoms were initially kept at on-lattice positions in the initial and final

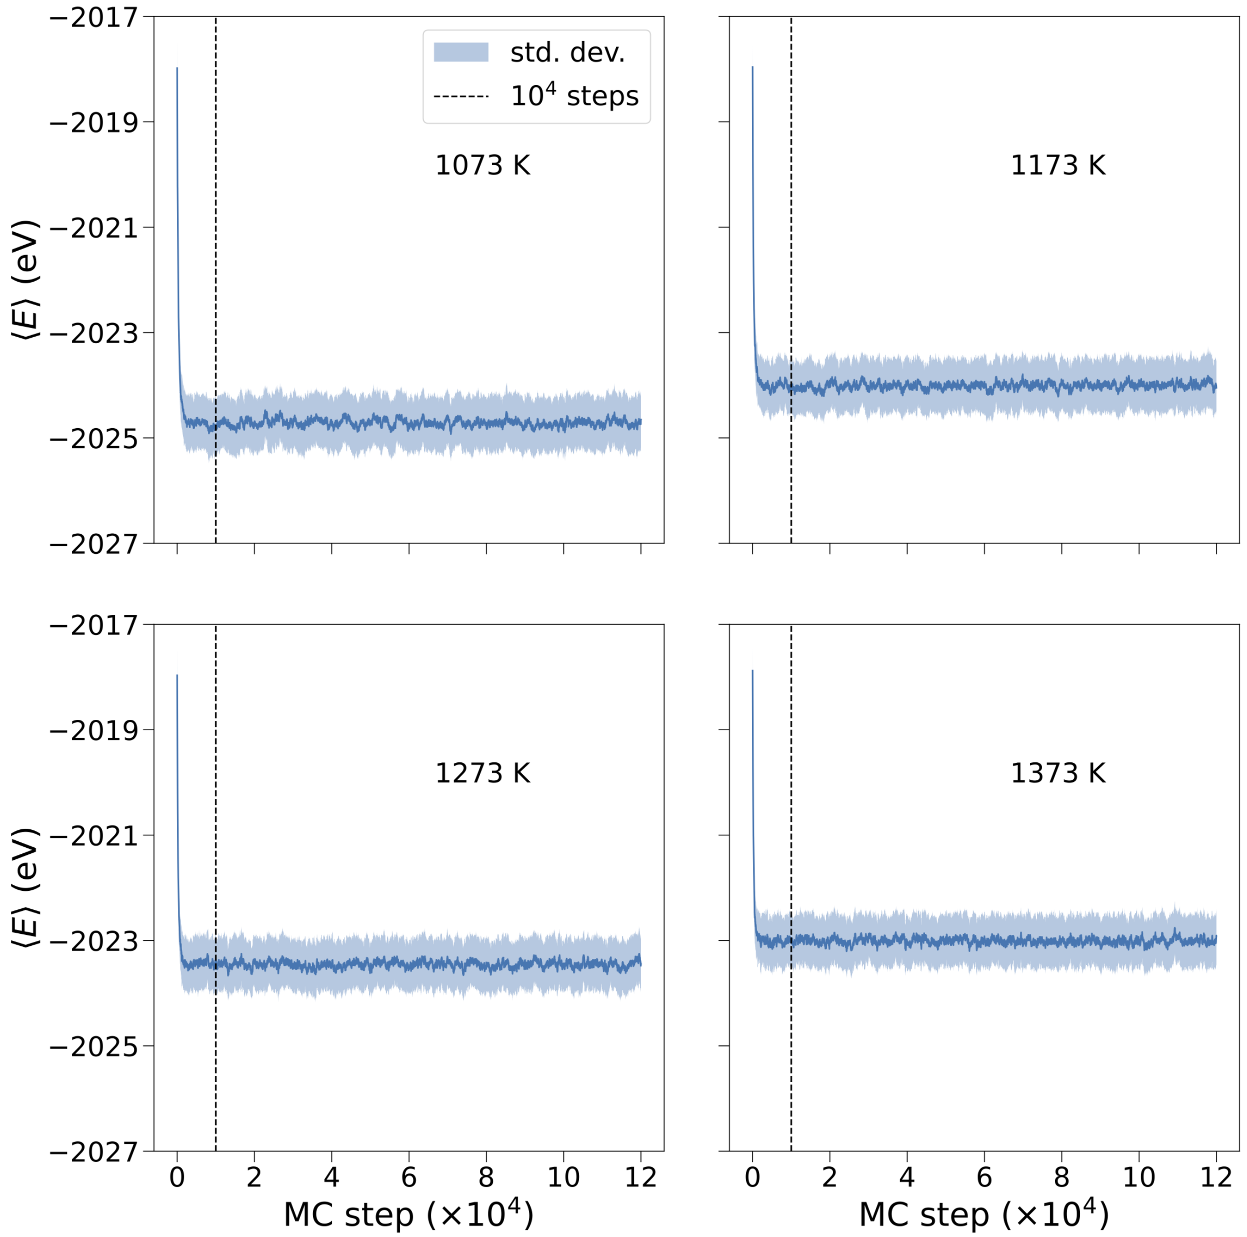


FIG. S3. Variation of the state energies as a function of Monte Carlo steps. At each step, the energies are reported as averages over 200 independent simulations, with the shaded region indicating one standard deviation about the mean energy at each step. After 10000 steps, reasonable convergence was achieved in the energies. States were gathered from the $10000^{th}$ step, at intervals of 1000 steps. 100 states were gathered from each independent simulation.

images, and the intermediate images were constructed using linear interpolation of the position of the jumping atom. A maximum force tolerance per atom of $10^{-3}$ eV/Å was used to relax each image. A tangential spring force of 10 eV/Å was applied to the images based on relative deviations from their initially assigned, equispaced positions on the band of images (LAMMPS

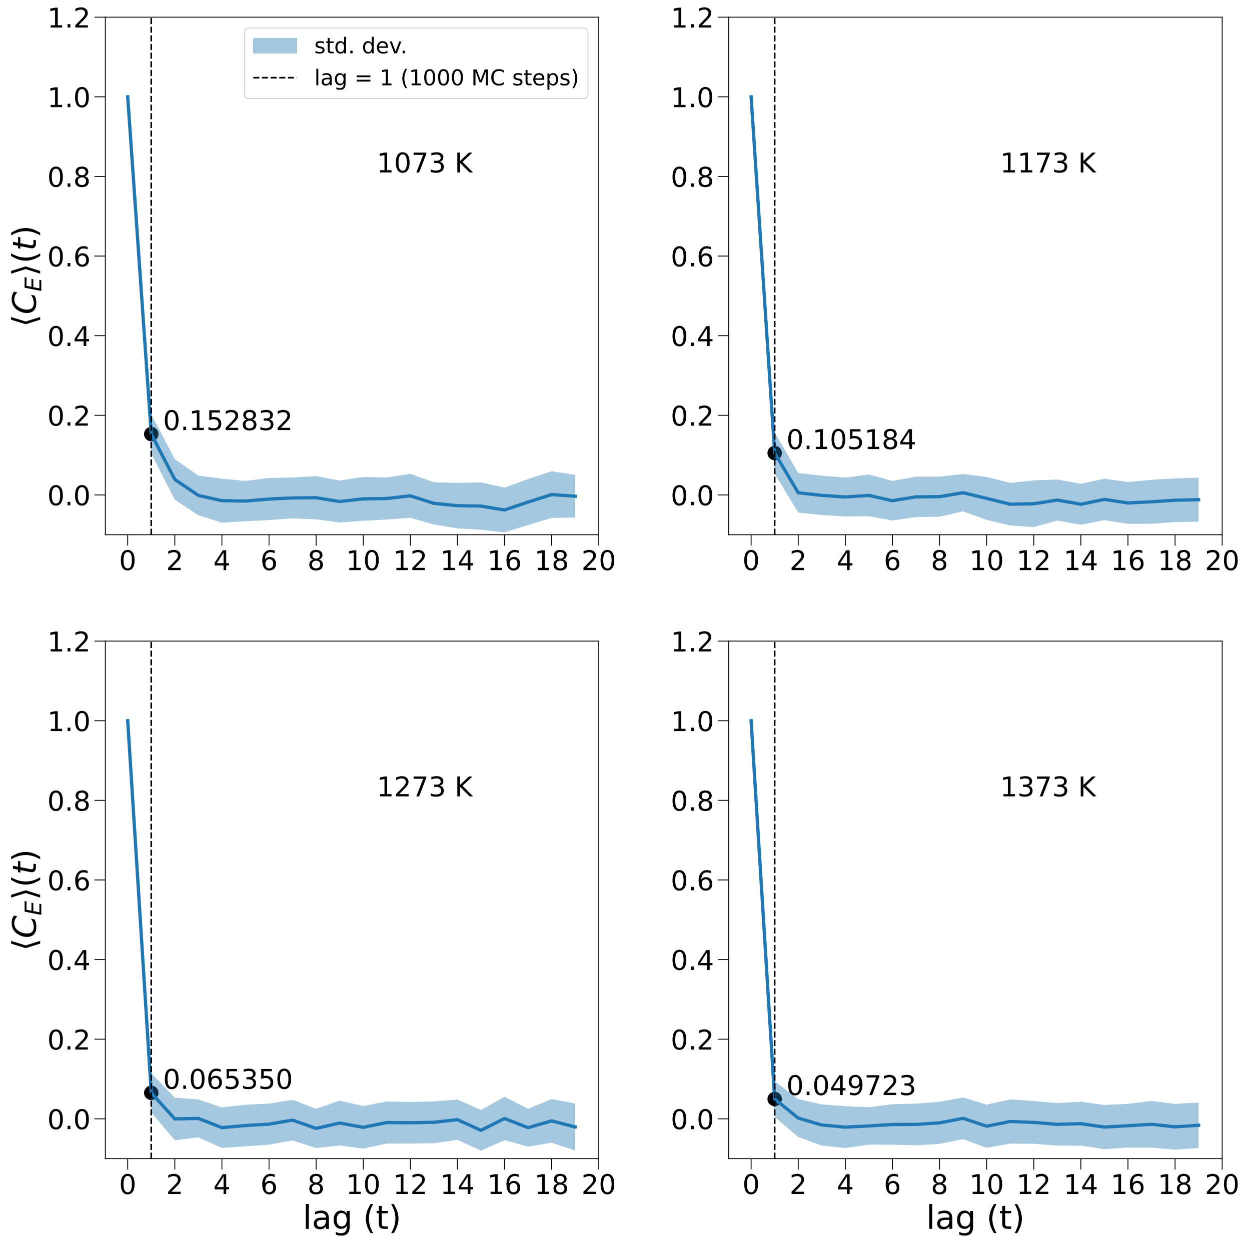


FIG. S4. Auto-correlation functions $C_E(t)$ of energies of the states gathered one after the other at intervals of 1000 MC steps, as a function of the lag (t) between such samples. Values were averaged across the 200 separate MC runs and the standard deviations at each $t$ for all four temperatures are indicated with the shaded regions. We find that statistical correlations in the state energies are reasonably small even at a lag of 1 (values indicated with the black dots), and quickly decay to zero which indicates sufficient independence of the samples gathered from our MC simulations.

keywords `parallel ideal` following [69]). An additional perpendicular spring force with a spring constant of 10 eV/Å$^2$ was also applied to prevent the formation of acute kinks in the band of images [70]. All relaxations during NEB calculations were carried out using the `ABCFIRE` algorithm for damped dynamics [71], with a starting time step of 0.001 picoseconds, a maximum

adaptive time step of 0.005 picoseconds (LAMMPS keyword `tmax 5.0` [72]), and a maximum allowed displacement of 0.01 Å per iteration, for a maximum of 20000 iterations.

For the construction of the datasets to predict diffusivities, a single KMC step was taken from the starting states using the barriers obtained from the NEB calculations and the KMC algorithm described in Section S2, and the rates out of the final state of the KMC step (states $\mathbf{n}'$ in Equation S2) were also computed. On occasion, attempted vacancy exchanges resulted in relaxation to unstable states. We rejected the following jumps:

1. Jumps to or from states with large atomic relaxations: Prior to the NEB calculation for any given vacancy-atom exchange, the initial and final atomic configurations were individually relaxed with a force tolerance of $10^{-3}$ eV/Å with the `ABCFIRE` algorithm. If the initial configuration of the first KMC step showed an atomic displacement from the lattice positions greater than a threshold of 1.0 Å, the corresponding sample was removed from the dataset. If the final configuration of any NEB calculation showed a similar displacement of any atom from its lattice site by more than 1.0 Å, jumps to such a configuration were blocked by setting the rate to 0.

2. Jumps to or from unstable states: If any of the initial or final states of a single KMC step was found to have a vacancy-atom exchange with a barrier less than 10 meV, the corresponding single-step KMC sample was removed from the dataset, as it was deemed to occur either to or from an unstable state.

3. Jumps breaking detailed balance: After computing the barriers of the jumps from both the initial ($\mathbf{n}$) and final ($\mathbf{n}'$) states of a single KMC step sample, if the transition state energy (obtained by adding the energy of the starting state to the barrier) for going from $\mathbf{n}$ to $\mathbf{n}'$ differed by more than 1 meV from that obtained while going back from $\mathbf{n}'$ to $\mathbf{n}$, the sample was removed from the dataset.

4. Large disagreements in state energies: If the energy of the first NEB image, corresponding to the starting atomic configuration of a vacancy-atom exchange, differed by more than 5 meV across the 12 NEB calculations for the 12 possible vacancy-atom exchanges in any of the initial or final states of a single KMC step sample, it was removed from the dataset. Such disagreements can happen if one or more of the 12 NEB calculations require substantially more iterations to converge than the others, or if the first image relaxes to substantially

different energy minima during the 12 NEB calculations. Similarly, if the minimum of the energies of the 12 first NEB images, obtained from the 12 NEB calculations from the initial state of a single KMC step sample, differed from the energy of the same state obtained during the MC simulations (using the CG algorithm) by more than 5 meV, the sample was also removed from the dataset.

Only a small fraction of the 20000 samples were removed from the datasets due to these deficiencies, with 19770, 19773, 19836 and 19811 samples remaining in the datasets for 1073 K, 1173 K, 1273 K and 1373 K respectively. Furthermore, out of these many samples that remained in the datasets, only 0.020%, 0.021%, 0.019%, 0.016% of the jumps (from either the initial or final states of the single KMC steps) had their rates set to 0 due to large atomic relaxations in the 1073 K, 1173 K, 1273 K and 1373 K respectively. This indicates sufficient robustness of the NEB calculations. Of these samples, 10000 were used for training the parametric models, and the remaining for validation. This may lead to a very small number of states entering both the training and validation sets from the same MC run.

The distribution of the vacancy-atom exchange barriers obtained from the initial and final states of the single KMC steps across the datasets of all four temperatures are shown in Figure S5. For the jumps out of the initial states, corresponding to the equilibrium barrier distribution, we find from the left figure in Figure S5, that all the species show approximately normal distribution of the barriers, with appreciable overlaps, as also seen elsewhere for the same potential [48, 49]. From the jumps out of the final states, we find from the distribution in the right figure in Figure S5, that almost all the species show a shift towards smaller migration barriers, indicating that the atomic neighborhoods in the initial states are more stable (under the reasonable assumption that more stable configurations would also have higher migration barriers).

To estimate the attempt frequencies of the various species needed to compute the jump rates along with the vacancy-atom exchange barriers, Vineyard's expression [9] within the "hopping-atom approximation" [73] was used. Following this method, the attempt frequency of a jump is computed as

$$\nu^0 = \frac{\prod_{i=1}^{3} \omega_i}{\prod_{i=1}^{2} \omega_i^{'}} \tag{S16}$$

where the vibrational frequencies $\omega_i$ are determined from the square roots of the eigenvalues of the dynamical matrix (computed using LAMMPS) of only the jumping atom in the initial state, and $\omega_i^{'}$ from the same at the transition state (the NEB image with the highest energy). In our calculations,

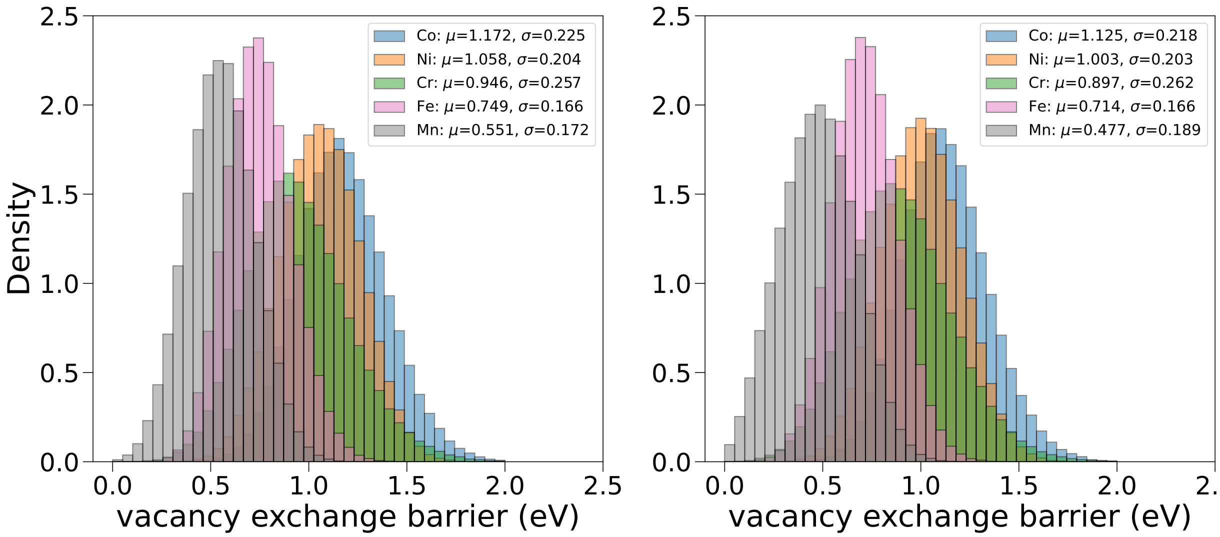


FIG. S5. Distribution of migration barriers for vacancy-atom exchange $E_b$ out of the initial (left) and final (right) states of single KMC steps obtained by Nudged Elastic Band calculations in the "Complex" rate system across the 1073 K, 1173 K, 1273 K and 1373 K datasets. The left figure corresponds to the equilibrium distribution of the barriers, and shows approximately normal distributions, with means ($\mu_b^\alpha$) and standard deviations ($\sigma_b^\alpha$) indicated for each species $\alpha$ (= Co, Ni, Cr, Fe, Mn). The right figure shows that from the final states of the single KMC steps, all the species tend to show smaller barriers than those encountered in the initial states, which can be due to energetic preference for the atomic neighborhoods in the initial states, which may be indicative of some ordering tendencies. These energy distributions are overall in agreement with that reported elsewhere for the same potential [47–49].

1000 initial states of single KMC steps were considered randomly from the datasets at each of the four temperatures, and a total of 40215 vacancy-atom exchange jumps were found from them that showed three real $\omega_i$ at the initial state, and two real $\omega_i^{'}$ at the transition state. The results of computing $\nu^0$ from these jumps using Equation S16 are shown in Figure S6. It is seen that all species have close attempt frequencies ranging from 22 to 30 THz, with considerable overlap in their distributions, due to which we assumed a constant value of 25.923 THz corresponding to the average over all 40215 samples.

After the datasets were constructed at each temperature for the "Complex" rate system, the diffusivities of the three fastest species, Mn, Fe, and Cr and that of the vacancy by optimizing the parametric models in Section S1 using Equation S2. To verify the diffusivities so obtained, full KMC simulations were also performed at each temperature up to 100 steps using the MEAM potential to compute all the necessary barriers via NEB calculations at each step using the same settings to construct the single KMC step datasets. The diffusivities in these full KMC simulations were averaged over 5000 such independent KMC trajectories, with the starting state of each

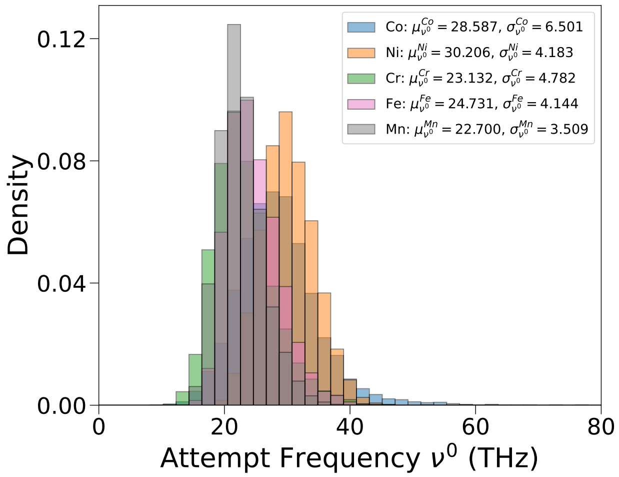


FIG. S6. Distribution of attempt frequencies $\nu^0$ of vacancy-atom exchange jumps computed using Vineyard's expression under the hopping atom approximation (Equation S16). A total of 40215 atomic jumps were simulated, consisting of 8652, 8172, 6393, 7177 and 9821 jumps of Co, Ni, Cr, Fe and Mn respectively, that showed three real vibrational frequencies at the initial states and two at the transition states. For each species $\alpha$ (= Co, Ni, Cr, Fe and Mn), the mean ($\mu^{\alpha}_{\nu^0}$) and standards deviation ($\sigma^{\alpha}_{\nu^0}$) are also indicated. It is seen that atoms with heavier atomic masses, such as Co and Ni, show larger mean attempt frequencies than lighter elements such as Mn, indicating stiffer atomic bonds for the heavy elements. Considerable overlap exists between the distributions for the different species; the attempt frequency of all vacancy-atom exchange jumps were taken to be the average value of 25.923 THz.

trajectory chosen randomly from the single KMC step datasets, shown in Figure 2 in our main paper.

A dataset of single KMC steps was generated at 773 K for the high entropy alloy as well; see Figure S7. Starting states were gathered from 200 independent MC simulations, starting at the $10000^{th}$ step, at intervals of 1000 steps. As seen to the left of Figure S7, this gives states that are reasonably equilibrated. After the states were gathered, an autocorrelation analysis of the state energies was performed. As seen to the right of Figure S7, a higher amount of correlation was observed in the states. The correlations still decay quickly, so our samples are uncorrelated. Migration barriers were computed from them using NEB calculations; samples were also rejected from this dataset as before; about 3.1% of the samples had to be rejected, and a dataset of 19379 single KMC step samples was produced.

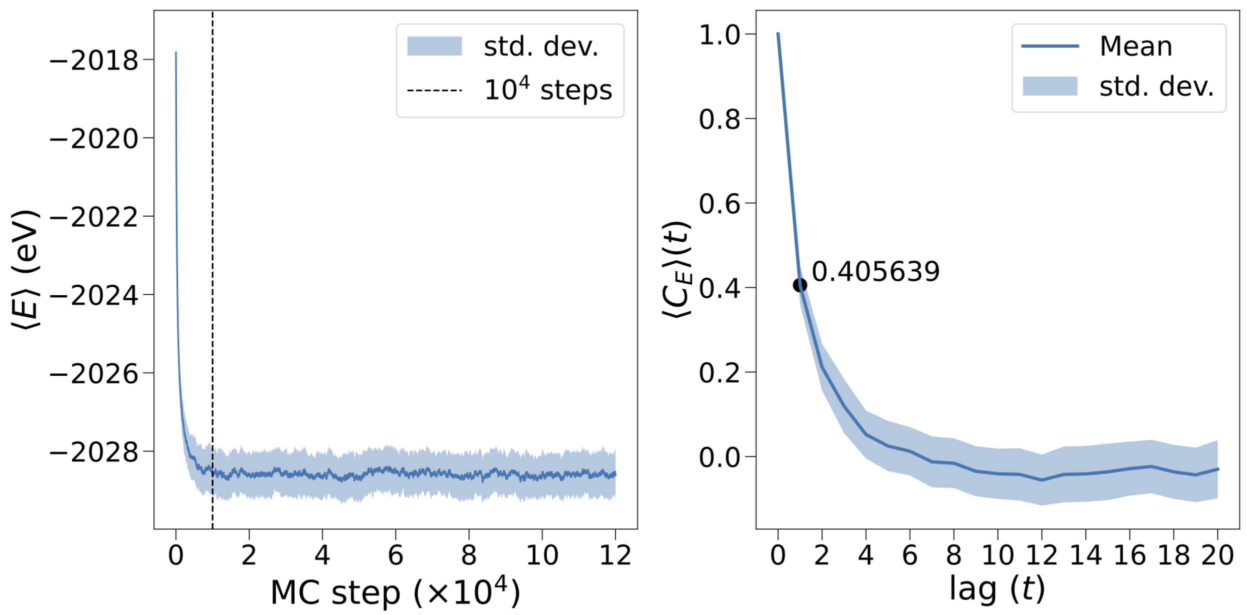


FIG. S7. Energy convergence as a function of MC steps (left) and autocorrelation function between states gathered from the MC simulation (right) at 773 K. All results are averages of 200 independent MC simulations, and the standard deviations are indicated by the shaded region. In the right figure, a lag of 1 corresponds to 1000 MC steps. It is seen that by 10000 steps, a reasonable convergence is achieved in the state energies. Higher correlations are observed between the states, however, due to lower acceptance rates of atomic swap trials during the MC runs. The correlations still decay to zero reasonably quickly, indicating sufficient independence of the samples.

## S5. CLUSTER EXPANSION AND NEURAL NETWORK MODEL SELECTION

The cluster expansion (CE) and network (NN) models have variable number of parameters; the size of these models serve as metaparameters to be optimized. The models were tested on the high entropy alloy and the "Ordered" rate 5-component systems datasets at 1173 K, and the "Ordered" rate 2-component systems at 80% atom concentration of the slow species. For fairness of comparison of model performance between the "Ordered" and "Random" rate systems, the optimal CE and NN models found were used on both.

Optimal cluster expansion models were selected by looking at their performance with variations in the largest allowed number of atoms and the maximum allowed range of separation between any pair of atoms in a cluster. These results are summarized in Figure S8. In general, it is found that increasing the cluster size as well as range of the clusters is necessary to improve diffusivity predictions. This highlights the fact that the relaxation vectors can be quite complicated functions of a state. With increase in the number of species, the number of clusters to consider also grows combinatorially and this leads to larger training-validation disagreements for the 5-component

"Ordered" rate and "Complex" systems compared to the "Ordered" rate 2-component system.

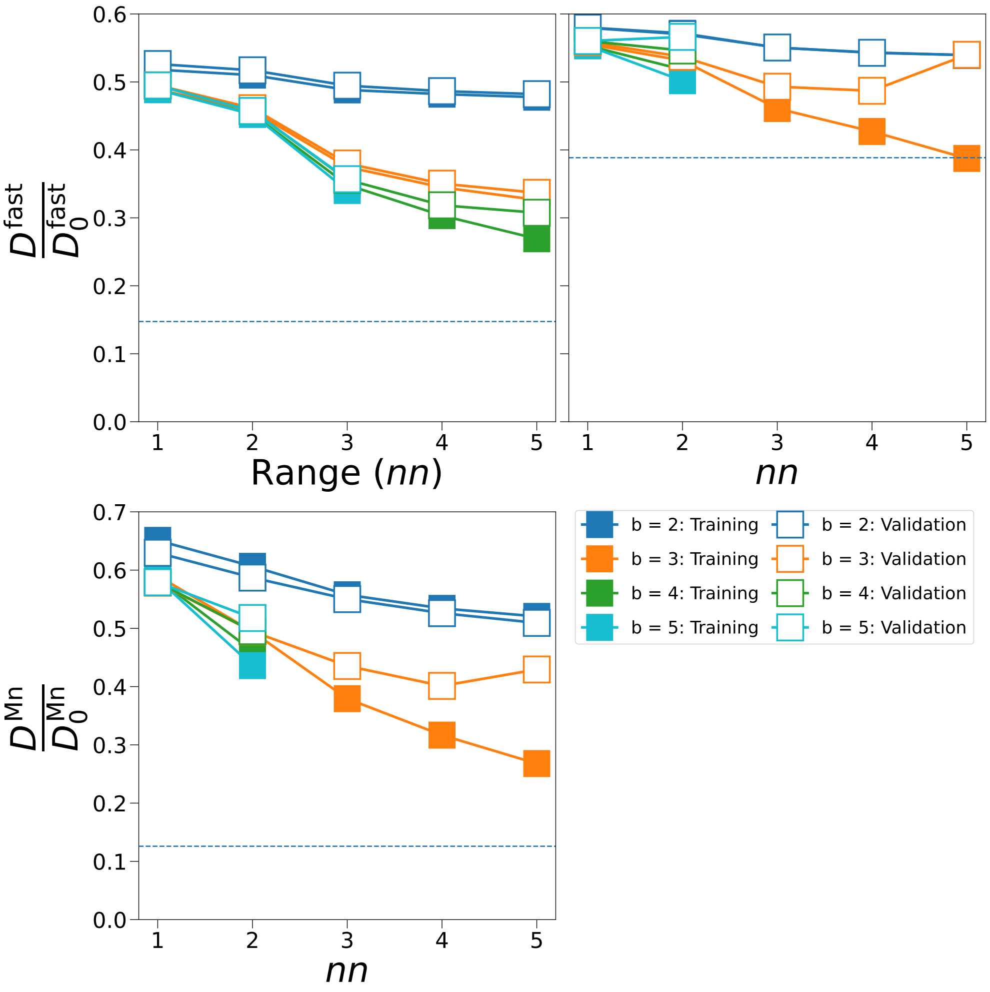


FIG. S8. Cluster expansion model performance with varying largest range of separation between any pair of atoms, measured in terms of nearest neighbors ($nn$), and cluster size, $b$ (maximum number of atoms in a cluster). Results are shown for the "Ordered" rate 2-component system at 80% slow species concentration (top left), and at 1173 K for the "Ordered" rate 5-component system (top right) and "Complex" rate (bottom left) systems. The diffusivity of the species with the fastest mean exchange rate with the vacancy ("fast" species for the "Ordered" rate systems and Mn for "Complex" rate system) was computed. The dotted horizontal lines show the values after 100 steps of KMC. The models with the least validation set diffusivity were selected. For the "Ordered" rate 2-component system system, it was the 4-body, $5^{\mathrm{th}}$ nearest neighbor CE model, while for the 5-component "Ordered" rate and "Complex" rate systems, it was the 3-body $4^{\mathrm{th}}$ nearest neighbor CE model.

To find optimal neural network models, the number of layers, and the number of channels in the intermediate layers between the input and output layers were varied. For simplicity, all such intermediate layers were constructed with a fixed number of input and output channels. For all of these studies, the neural networks were trained up to a maximum of 5000 epochs, evaluated every

10 epochs, and the minimum diffusivity achieved on the validation set and the corresponding value on the training set were recorded. The results of this study are summarized in Figure S9. For the 5-component systems, the prediction performance saturates at 3 intermediate layers, while for the "Ordered" rate 2-component system, the performance continues to improve even up to 6 intermediate layers.

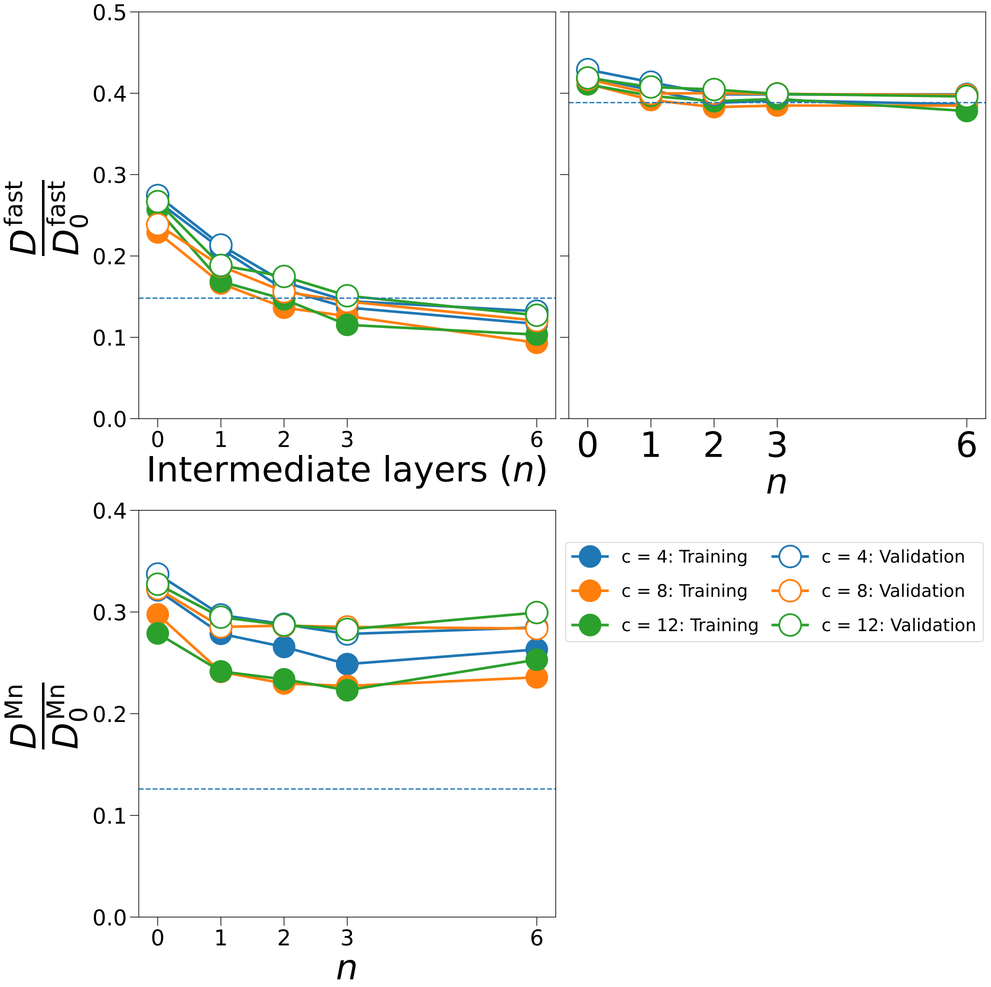


FIG. S9. Neural network performance with varying number of intermediate layers ($n$), i.e, excluding the input and output layer, each having $c$ input and output channels. Results are shown for the "Ordered" rate 2-component system system at 80% slow species concentration (top left), and at 1173 K for "Ordered" rate 5-component system system (top right) and the "Complex" rate system (bottom left). For each system, the diffusivity of the species with the fastest mean exchange rate with the vacancy ("fast" species for the "Ordered" rate systems and Mn for the "Complex" rate system) was computed. For each neural network, training was done for 5000 epochs, diffusivities calculated every 10 epochs and the size with the minimum validation set diffusivity was considered the optimal choice. For the "Ordered" rate 2-component system the network configuration with 6 intermediate layers and 8 channels, for the "Ordered" rate 5-component system the network configuration with 3 intermediate layers and 8 channels, and for the "Complex" rate system the network configuration with 3 intermediate layers and 4 channels were selected.

## S6. NEURAL NETWORK TRAINING

Training curves for the “Ordered” rate systems (2 and 5-component) are in Figure S10 and Figure S11; each epoch corresponding to one sweep of gradient descent steps across the whole training set, which was found to provide sufficient convergence. Training curves for the high entropy alloy are shown in Figure S12, the networks were trained up to a maximum of 60000 epochs by which the validation sets show a minimum at all temperatures. The networks were evaluated every 10 epochs, and the minimum diffusivity obtained on the validation set, with the corresponding value on the training set were taken as the optimal values. The final diffusivity comparison is in Figure S13.

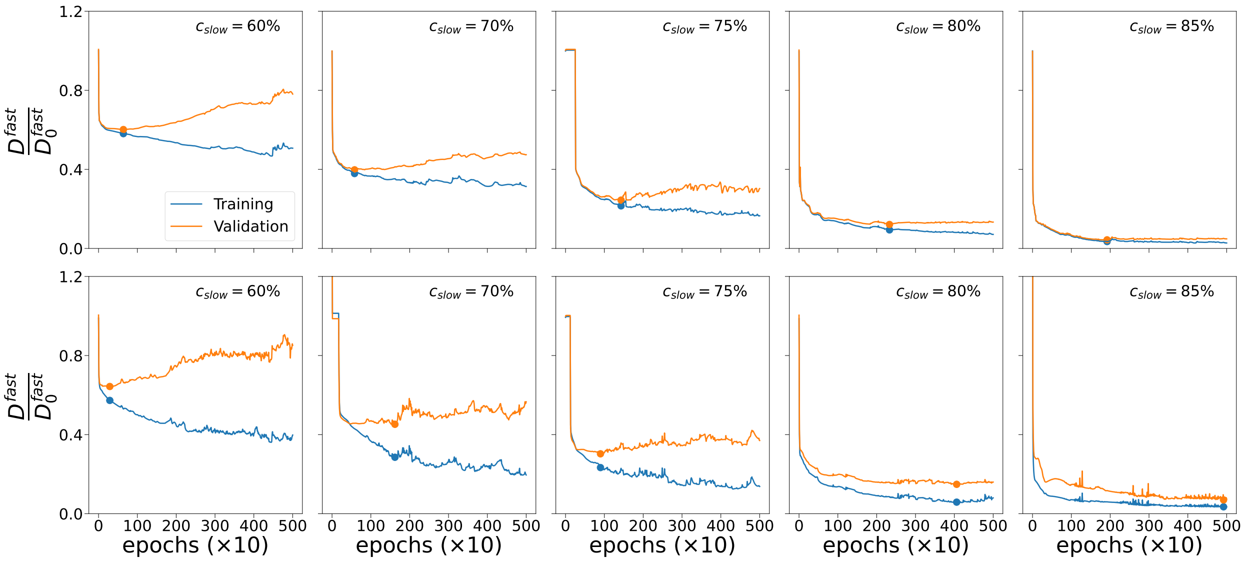


FIG. S10. Evolution of neural network diffusivity prediction for the “fast” species in the 2-component “Ordered” (top row) and “Complex” (bottom row) rate systems. All networks had 6 intermediate layers, with 8 channels per layer and were trained to a maximum of 5000 epochs and evaluated every 10 epochs. The blue and orange circles indicate the optimal training and validation set diffusivities, corresponding to the minimum observed value in the validation set.

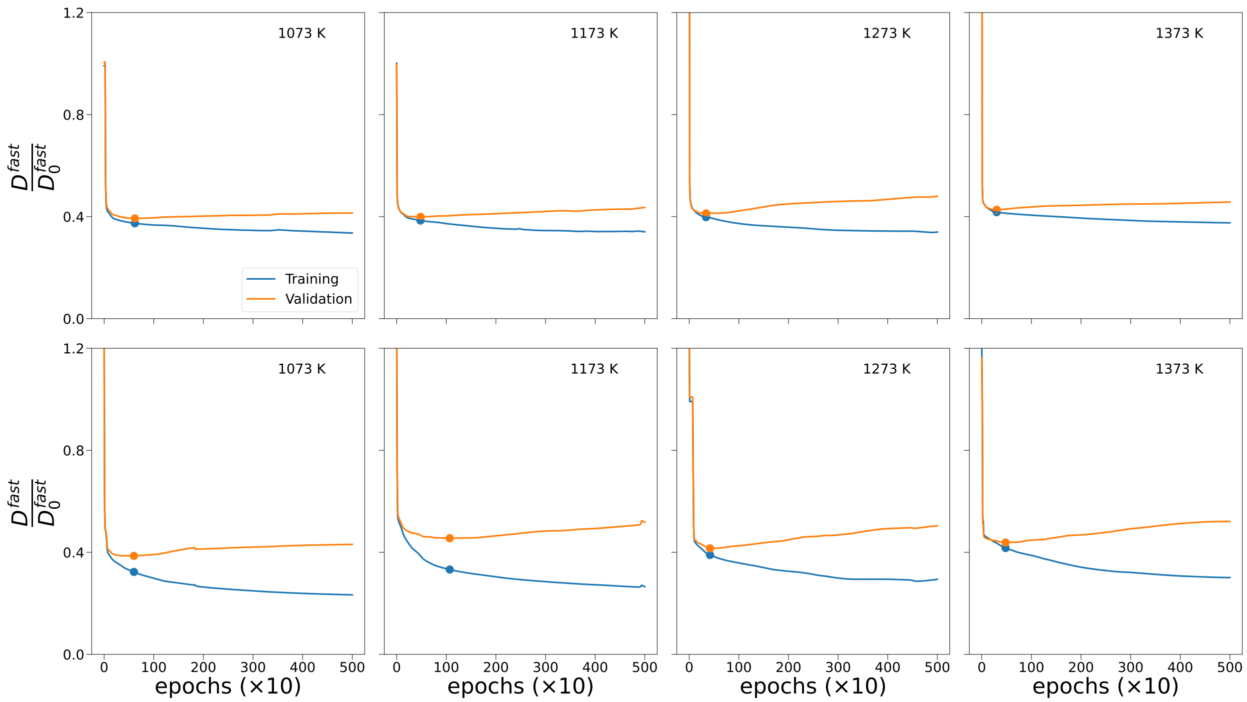


FIG. S11. Evolution of neural network diffusivity prediction for the "fast" species in the 5-component "Ordered" (top row) and "Complex" (bottom row) rate systems. All networks had 3 intermediate layers, with 8 channels per layer and were trained to a maximum of 5000 epochs and evaluated every 10 epochs. The blue and orange circles indicate the optimal training and validation set diffusivities, corresponding to the minimum observed value in the validation set.

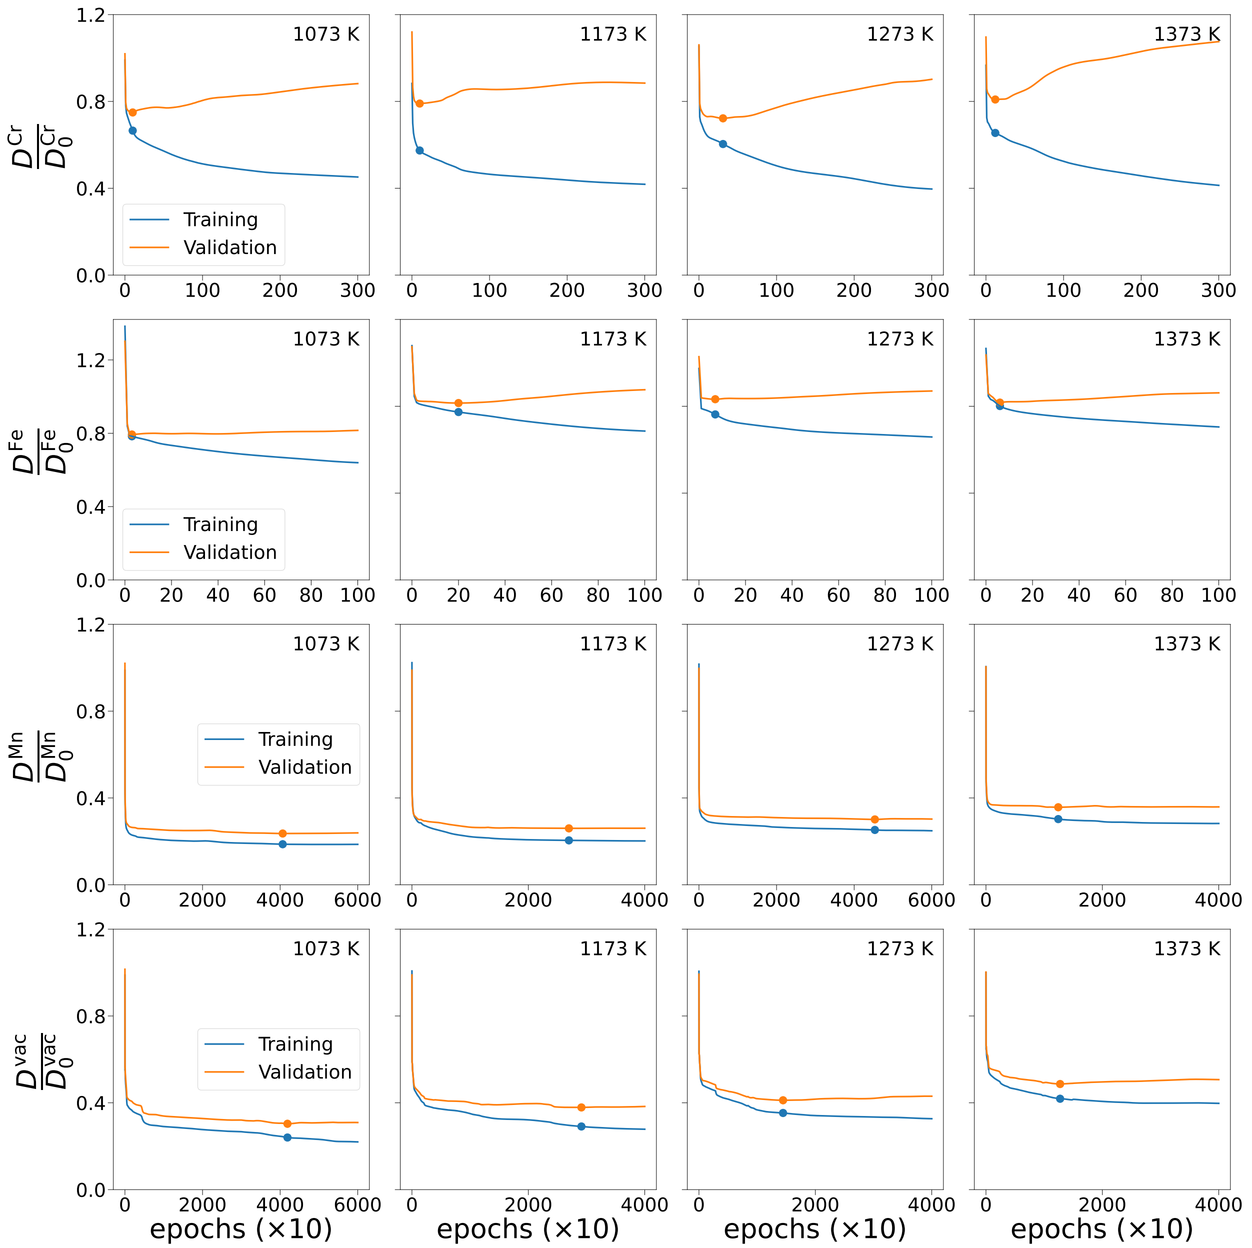


FIG. S12. Evolution of Neural network diffusivity prediction for the four fastest species (Cr, Fe, Mn and the vacancy) in the high entropy alloy. All networks had 3 intermediate layers with 4 channels per layer, and were trained to a maximum of 60000 epochs and evaluated every 10 epochs. The blue and orange circles indicate the optimal training and validation set diffusivities, corresponding to the minimum observed value in the validation set.

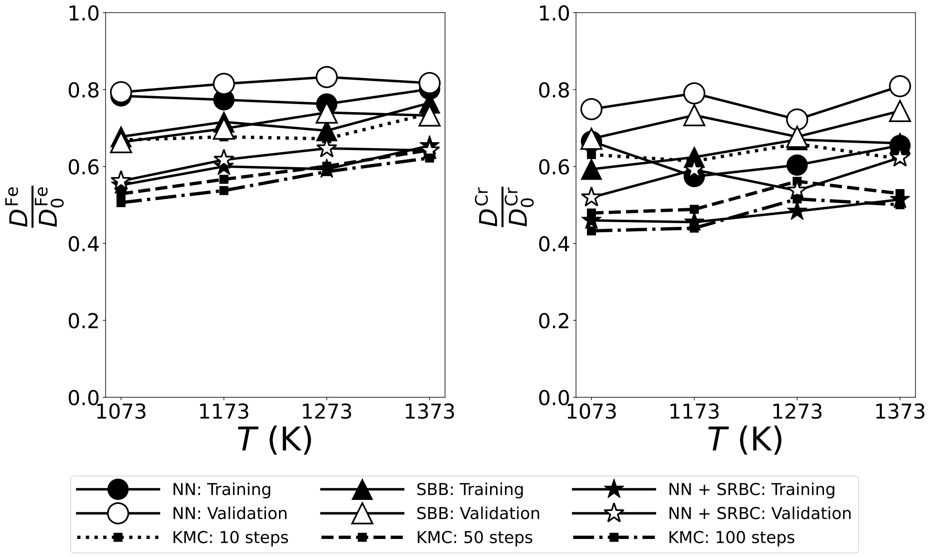


FIG. S13. Predicting Fe (left) and Cr (right) diffusivity in a five component high entropy alloy. Diffusivity is shown as a fraction of the one-step diffusivity prediction; with smaller values indicating increased trapping.

## S7. SRO AT 773 K

In order to using our NN model trained at high temperature to lower temperatures, we evaluated short range ordering parameters in our high enetropy alloy. We measure the SRO parameter between two species $\alpha$ and $\beta$ as

$$\mathrm{SRO}^{\alpha\beta} = \frac{\left\langle N^{\alpha\beta} \right\rangle - N^{\alpha\beta}_{\mathrm{random}}}{N^{\alpha\beta}_{\mathrm{max}} - N^{\alpha\beta}_{\mathrm{random}}} \tag{S17}$$

This expression is similar to those found in [47, 74]. Here, $\left\langle N^{\alpha\beta} \right\rangle$ corresponds to the number of nearest neighbor bonds between two species $\alpha$ and $\beta$ in a state, averaged over the whole dataset of the starting (equilibrium) states of single KMC steps at any given temperature. The quantities $N^{\alpha\beta}_{\mathrm{max}}$ and $N^{\alpha\beta}_{\mathrm{random}}$ are the maximum number of such bonds, and that found in a perfectly random alloy respectively. These are given by [47]

$$N^{\alpha\beta}_{\mathrm{max}} = Nzc_\alpha,\ \alpha \neq \beta \tag{S18}$$

$$N^{\alpha\alpha}_{\mathrm{max}} = \frac{1}{2} Nzc_\alpha \tag{S19}$$

$$N^{\alpha\beta}_{\mathrm{random}} = Nzc_\alpha c_\beta,\ \alpha \neq \beta \tag{S20}$$

$$N^{\alpha\alpha}_{\mathrm{random}} = \frac{1}{2} Nzc_\alpha c_\alpha \tag{S21}$$

where $N = 500$ is the number of lattice sites, $z = 12$ the number of nearest neighbors, and $c_\alpha = 0.2$ the atom fraction of species $\alpha$. A value of 0 for the SRO parameter in Equation S17 indicates perfect randomness. The results of the SRO parameter calculations are given in Table S2. At 1073 K, the values mostly appear within the range of those found in [47]. As mentioned in [47], for an equiatomic 5-component FCC system, a SRO of –0.25 (obtained by setting $\left\langle N^{\alpha\beta} \right\rangle = 0$ in Equation S17) between two species $\alpha$ and $\beta$ would indicate repulsive ordering, where no $\alpha$ atom has a $\beta$ atom as a nearest neighbor, while a value of 1.0 (obtained by setting $\left\langle N^{\alpha\beta} \right\rangle = N^{\alpha\beta}_{\mathrm{max}}$ in Equation S17) would indicate "clustering", where $\alpha$ atoms always have $\beta$ atoms as nearest neighbors. The values of the SRO parameter in Table S2 are closer to zero from these two extremes but are also appreciably different from the values in "Random" rate 5-component lattice gas (where

TABLE S2. Short range ordering parameters (SRO from Equation S17) in the high entropy alloy. In every cell, the values at 773 K, 1073 K, 1173 K, 1273 K and 1373 K are given one after the other from top to bottom and comma-separated. For a completely random system, these values would be 0. Values more negatively or positively away from 0 indicate repulsive or attractive ordering respectively. Some partial ordering is observed at all temperatures, in agreement with a similar observation in [48].

| | vac | Co | Ni | Cr | Fe | Mn |
|---|---|---|---|---|---|---|
| vac | 0, 0, 0, 0, 0 | – | – | – | – | – |
| Co | –0.010, 0.005, 0.003, 0.004, 0.004 | 0.017, 0.002, 0.000, –0.002, –0.003 | | | | |
| Ni | –0.009, –0.016, –0.016, –0.014, –0.014 | –0.019, –0.018, –0.017, –0.016, –0.015 | –0.039, –0.034, –0.033, –0.031, –0.030 | | | |
| Cr | 0.038, 0.003, 0.000, –0.005, –0.006 | –0.100, –0.054, –0.047, –0.041, –0.037 | –0.012, –0.002, –0.001, –0.001, –0.001 | 0.193, 0.096, 0.081, 0.071, 0.062 | | |
| Fe | –0.113, –0.070, –0.063, –0.058, –0.052 | 0.095, 0.060, 0.054, 0.049, 0.045 | 0.012, 0.010, 0.009, 0.009, 0.008 | –0.119, –0.067, –0.058, –0.051, –0.046 | 0.035, 0.010, 0.006, 0.004, 0.002 | |
| Mn | 0.094, 0.079, 0.076, 0.073, 0.068 | 0.002, 0.005, 0.005, 0.005, 0.005 | 0.053, 0.040, 0.037, 0.034, 0.032 | 0.033, 0.022, 0.020, 0.018, 0.017 | –0.027, –0.018, –0.016, –0.015, –0.013 | –0.066, –0.054, –0.051, –0.049, –0.046 |

a maximum magnitude of 0.003 of the SRO parameters was found), indicating some amount of ordering, particularly at 773 K. We note however, that the SRO values at 773 K are not too different from the other temperatures, compared relative to these extremes.

## S8. KINOSON DENSITIES

From Equation S2, the negative logarithm of the individual contribution by a single KMC step from any randomly sampled starting state $\mathbf{n}$ towards $2dD^{\alpha}$ for some species $\alpha$ is

$$-\ln(\kappa) := \ln \tau_{\mathbf{n}} - 2\ln(|\delta \mathbf{x}^{\alpha}(\mathbf{n} \rightarrow \mathbf{n}') + \mathbf{y}^{\alpha,*}_{\mathbf{n}'} - \mathbf{y}^{\alpha,*}_{\mathbf{n}}|) \tag{S22}$$

We scale the kinosons by the fundamental unit of diffusivity, $a_0^2\nu^0/2d$, where the lattice parameter $a_0 = 3.595$Å and the attempt frequency $\nu^0 = 25.923$ THz. The distributions of $-\ln(\kappa)$ (kinoson densities) for the vacancy are plotted in the top row of Figure 3 in the main text for varying levels of approximation for the relaxation vectors. From this figure, it is seen that the uncorrelated diffusivity contributions, for which the second term in the RHS of Equation S22 is a constant (corresponding to the nearest neighbor distance), follow an approximately normal distribution and as the relaxation approximations become more accurate, the distributions skew towards smaller values. From the bottom row of Figure 3, we find that the relaxed displacements show a decaying nature from a peak value of zero for vacancy–Mn exchange jumps, which constitute a majority ($\approx$ 80%) of sampled single-step KMC jumps in our datasets. From these observations, the "Exponentially Modified Gaussian" (EMG) distribution [51, 53] (or "Ex-Gaussian" distribution [52]), which describes the sum $Z = (X + Y)$ of a Gaussian distributed random variable, $X$, with an independent exponentially distributed one, $Y$, was examined for approximating the diffusivity contributions, owing to a similarity in form with Equation S22. The probability density function for this distribution is given as [53]

$$g(z) = \frac{\lambda}{2}\exp\left(\frac{\lambda^2\sigma^2}{2} + \lambda\mu - z\lambda\right)\mathrm{erfc}\left(\frac{\lambda\sigma^2 + \mu - z}{\sigma\sqrt{2}}\right) \tag{S23}$$

where $\mu$ and $\sigma$ correspond to the mean and standard deviation of the Gaussian $X$ and $\lambda$ is the decay rate for $Y$, and "erfc" denotes the complementary error function. As shown in Figure 3, for the case of vacancy diffusivity, the EMG distribution approximatew the individual contributions towards towards $2dD^{\alpha}$ from the dataset.

In order to assess the applicability of the EMG distribution towards other species, we also examined the kinoson densities of the three fastest atomic species in the dataset, namely Mn, Fe and Cr. These results are plotted in Figure S14. It was found that while the distributions of $-\ln(\kappa)$ show a positive skewness for the case of the vacancy and Mn, for Fe and Cr (which are slower

TABLE S3. Observed skewness for the distribution of $-\ln(\kappa)$ in Equation S22 for the vacancy, Mn, Fe and Cr obtained using NN+SRBC to approximate the relaxation vectors in the single-step KMC datasets for 1073–1373 K. For the EMG distribution the skewness must be positive and at most 2 [52]. Vacancy and Mn show positive skewness, while Fe and Cr show negative skewness. As such, for Fe and Cr, the normal distribution was used which neglects the skewness of the data. It is worth noting that as the temperature increases, the skewness becomes more positive, indicating excitation of Kinosons with larger diffusivity contributions with increasing temperature.

| | 1073 K | 1173 K | 1273 K | 1373 K |
|---|---|---|---|---|
| vacancy | 0.23157 | 0.270749 | 0.417981 | 0.493236 |
| Mn | 0.301064 | 0.345489 | 0.443698 | 0.467608 |
| Fe | -0.232186 | -0.233218 | -0.208803 | -0.131466 |
| Cr | -0.487312 | -0.489152 | -0.409167 | -0.367797 |

diffusers), these contributions show negative skewness as shown in Table S3. Since the EMG distribution only allows positive skewness, the densities for Fe and Cr were approximated with only the Gaussian distribution in the present study (corresponding to $\lambda^{-1} = 0$, which neglects the skewness of the data. We note, however, that all the skewness values observed were less than 0.5 in magnitude, indicating light tails in the data.

For all of these approximations mentioned above, the parameters $\mu$, $\sigma$, and $\lambda$ are obtained using a modified method-of-moments approach. We use the total diffusivity, the sample variance and skewness of the log of the distribution. For sample variance $s^2$ and skewness $\gamma_1$, the $\sigma$ and $\lambda$ parameters are

$$\sigma^2 = s^2\left[1 - \left(\frac{\gamma_1}{2}\right)^{2/3}\right] \tag{S24}$$

and

$$\lambda^{-1} = s\left(\frac{\gamma_1}{2}\right)^{1/3} \tag{S25}$$

following standard method-of-moments. The mean $\mu$ of the Gaussian distribution was chosen to reproduce $2dD^\alpha$ from the datasets (in units of $a_0^2\nu^0$). For the vacancy and Mn, the fitted $\mu$ can then be written as

$$\mu = -\ln(2dD^\alpha) - \ln\left(1 + \lambda^{-1}\right) + \frac{\sigma^2}{2} \tag{S26}$$

while for Fe and Cr, $\lambda^{-1} = 0$.

The reliability of these approximations were assessed in two ways. First, for the vacancy, Mn, Fe and Cr, we compared the empirical cumulative density function (CDFs) of $-\ln\kappa$ in Equa-

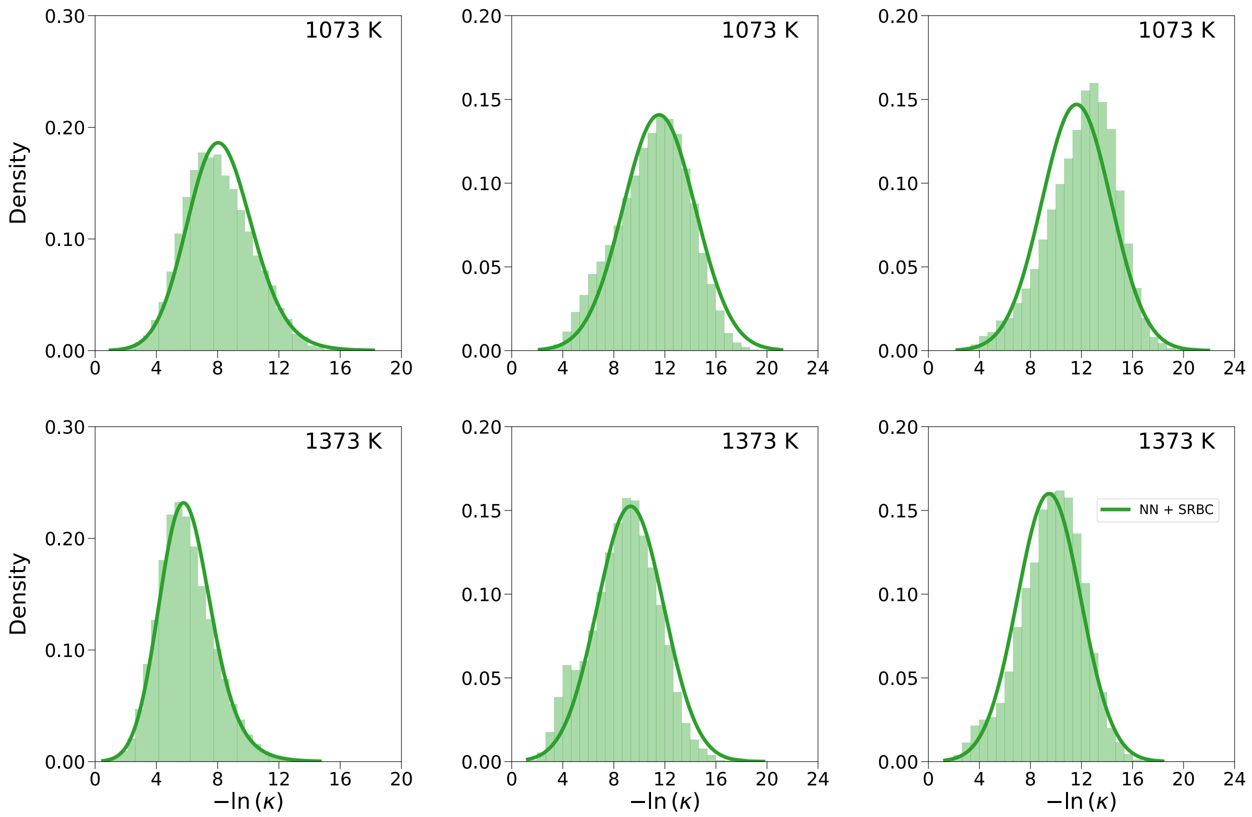


FIG. S14. Kinoson density for Mn, Fe and Cr obtained with the NN+SRBC scheme (Equation S13). Displacements are taken in units of the lattice parameter, 3.595Å, while the rates are measured in units of the attempt frequency, 25.923 THz (Figure S6). Mn was well-approximated with EMG, while for Fe and Cr, normal distribution worked better in lieu of EMG due to negative skewness in the data.

tion S22 from the datasets at 1073–1373 K for 100 quantiles and compared them with the theoretical cumulative densities obtained from the fitted distributions at each temperature. These results are plotted in Figure S15. There are small systematic mismatches between the data and the fitted theoretical distributions, with the RMS values of the disagreements no larger than 4.3% in the cumulative probabilities observed for Cr in the 1073 K dataset (as expected from Figure S14).

Second, we also used the fitted distributions to determine the diffusivity with temperature and then extrapolate the diffusivity to 773 K. The results were then compared with the diffusivity obtained from the single-step KMC dataset constructed at 773 K, using the neural networks trained on the 1073 K dataset and corrected with the SRBC scheme. From the temperature dependence of the parameters, the vacancy diffusivity can be extrapolated from the EMG distribution as per Equation 5 in our main text. For Mn, the extrapolated diffusivity follows a similar equation given

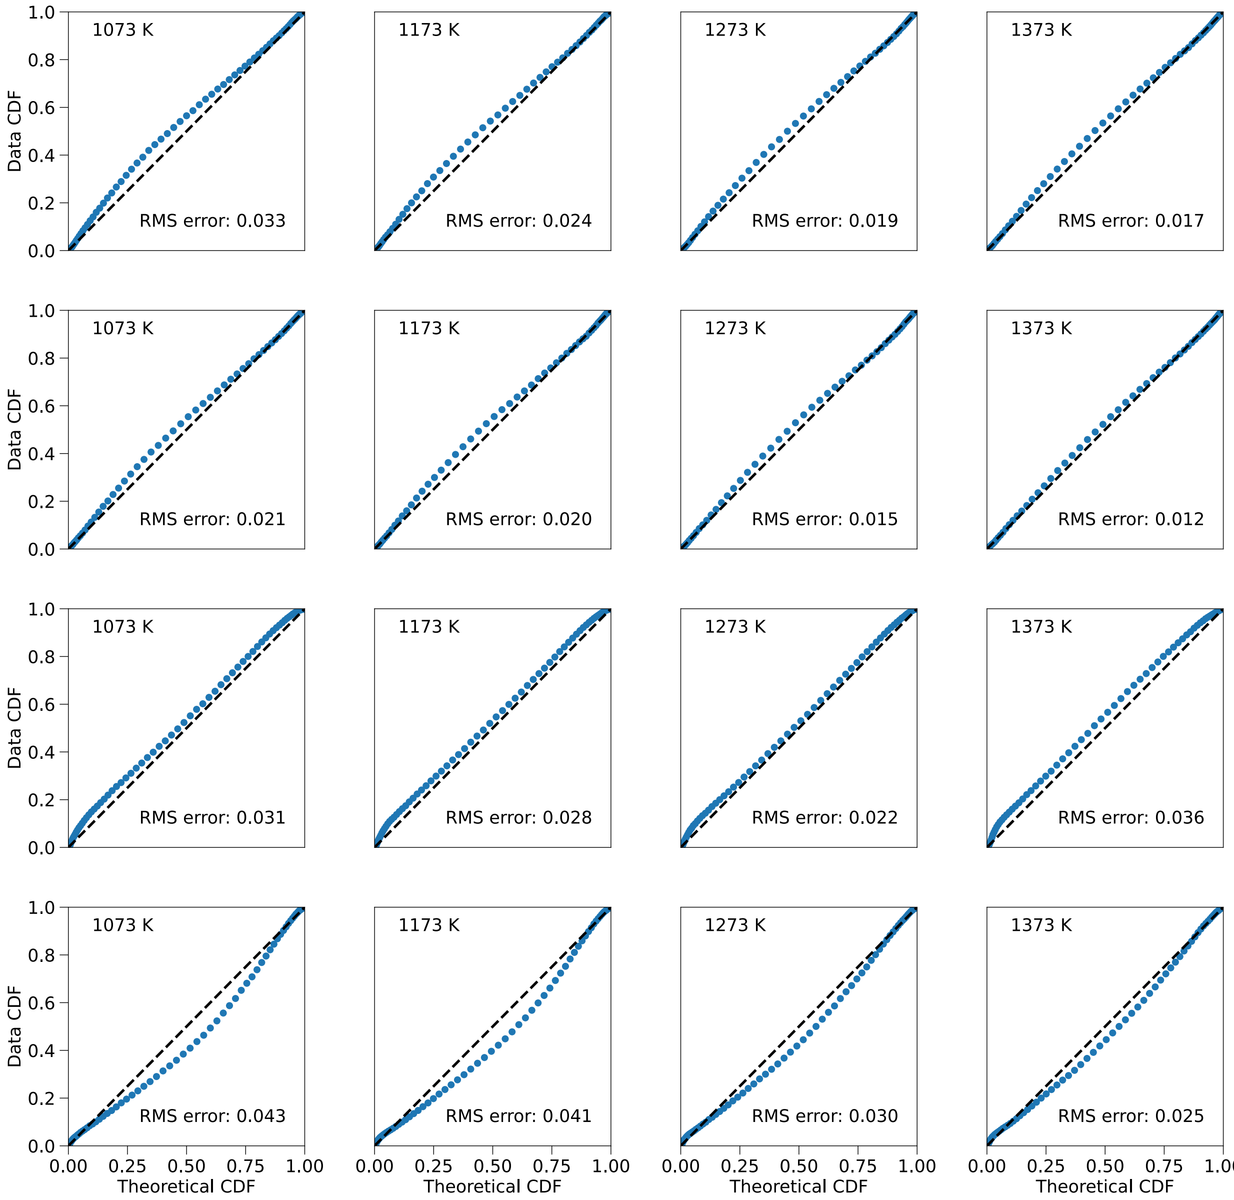


FIG. S15. Comparison of the observed cumulative kinoson densities (vertical axes) with the theoretical cumulative densities obtained from the fitted distributions (horizonatal axes) for 100 quantiles of the single-KMC step datasets from 1073 to 1373 K. In each case, the root-mean-square (RMS) disagreements between the two are also indicated, with the diagonal dotted lines indicating perfect agreement. From top to bottom, each row corresponds to the vacancy, Mn, Fe and Cr respectively. The plots show the existence of some systematic mismatch between the fitted distributions and the actual data. However, the disagreements are small, with the largest RMS error being 4.3% for Cr at 1073 K.

as

$$D^{(\mathrm{EMG})} = c_{\mathrm{v}} \left( \frac{\nu^0 a_0^2}{6} \right) \frac{\lambda}{\lambda + 1} \exp\left( -\mu + \frac{1}{2}\sigma^2 \right) \tag{S27}$$

with $a_0$ and $\nu^0$ being the lattice parameter and attempt frequency respectively, $c_{\mathrm{v}}$ being the vacancy

concentration, taken as $\exp(-E_{\mathrm{v}}^{f}/k_B T)$, with $E_{\mathrm{v}}^{f} = 1.72$ eV being the vacancy formation enthalpy in the Cantor alloy [75]. $\mu$ and $\sigma$ correspond to the mean and standard deviation of the Gaussian part and $\lambda$ being the decay rate of the exponential part of the EMG distribution. For Fe and Cr, the diffusivity expression becomes

$$D^{(\mathrm{Gaussian})} = c_{\mathrm{v}}\left(\frac{\nu^0 a_0^2}{6}\right)\exp\left(-\mu + \frac{1}{2}\sigma^2\right) \tag{S28}$$

For the vacancy, these results are shown in Figure 4 in the main text, and in Figure S16 for Mn, Fe and Cr. We find from these figures that the empirical extrapolation of the diffusivity agrees well with the neural network results, indicating reasonable approximation of the kinoson densities with the fitted distribution.

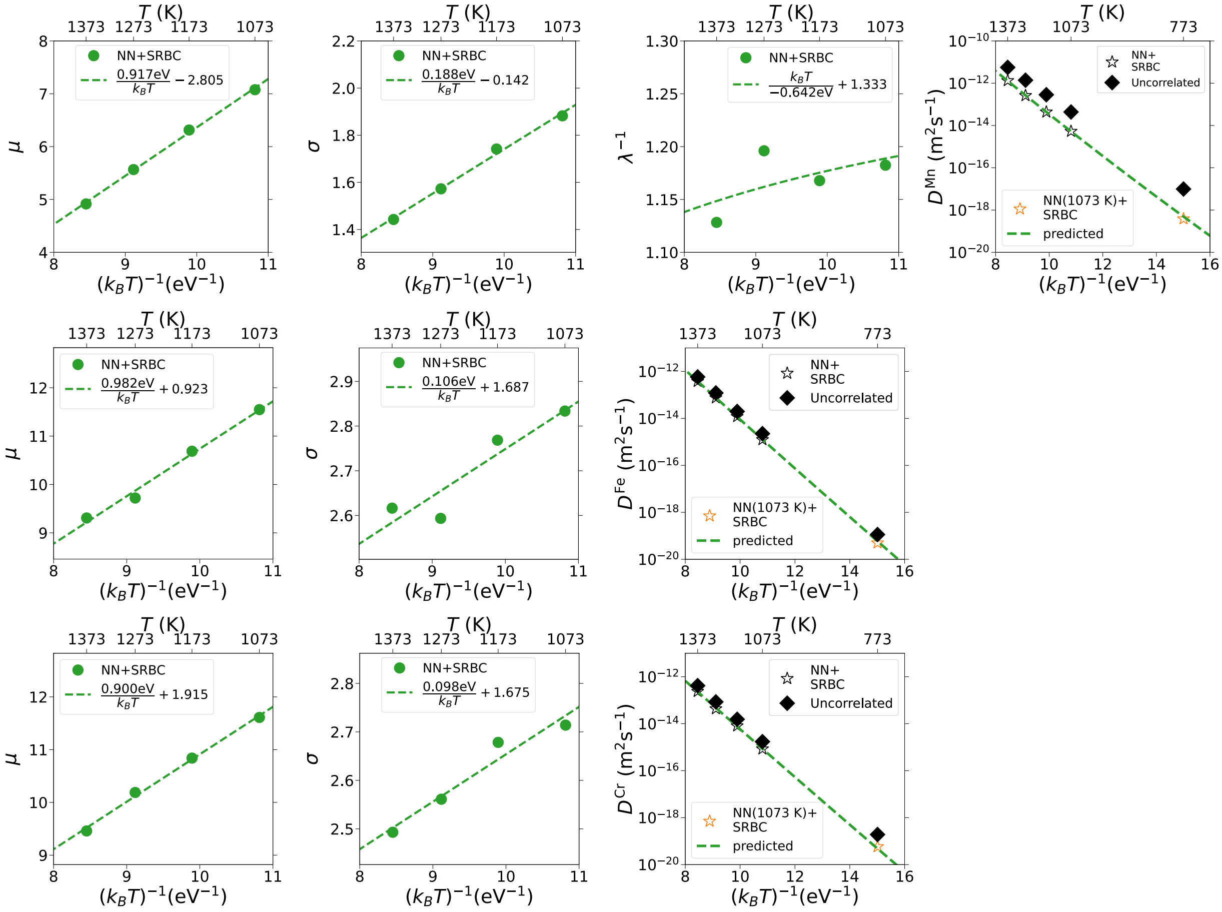


FIG. S16. Extrapolation of element diffusivities based on temperature variation of paramters governing empirical kinoson densities. The top row corresponds to results for Mn, the middle row for Fe and the bottom row for Cr.

[1] A. Fick, Annalen der Physik **170**, 59 (1855), https://onlinelibrary.wiley.com/doi/pdf/10.1002/andp.18551700105.

[2] A. Einstein, Ann. d. Physik **322**, 549 (1905).

[3] L. Onsager, Phys. Rev. **37**, 405 (1931).

[4] W. C. Roberts-Austen, Philos. Trans. Royal Soc. London A **187**, 383 (1896).

[5] R. W. Balluffi, S. M. Allen, and W. C. Carter, *Kinetics of Materials* (John Wiley & Sons, Inc., 2005).

[6] S. Arrhenius, Z. Phys. Chem. **4U**, 226 (1889).

[7] H. Eyring, J. Chem. Phys. **3**, 107 (1935).

[8] M. G. Evans and M. Polanyi, Trans. Faraday Soc. **31**, 875 (1935).

[9] G. H. Vineyard, J. Phys. Chem. Solids **3**, 121 (1957).

[10] P. Heitjans and J. Kärger, *Diffusion in Solids: Fundamentals, Methods, Materials, Diffusion-Controlled Processes*, Springer Series in Solid-State Sciences (Springer-Verlag Berlin Heidelberg, 2005).

[11] H. Mehrer, *Diffusion in Solids: Fundamentals, Methods, Materials, Diffusion-Controlled Processes*, Springer Series in Solid-State Sciences (Springer-Verlag Berlin Heidelberg, 2007).

[12] G. E. Murch, in *Diffusion in Crystalline Solids*, edited by G. E. Murch and A. S. Nowick (Orlando, Florida: Academic Press, 1984) Chap. 7, pp. 379–427.

[13] I. V. Belova and G. E. Murch, Philos. Mag. A **80**, 599 (2000).

[14] I. V. Belova and G. E. Murch, Philos. Mag. A **81**, 1749 (2001).

[15] I. V. Belova and G. E. Murch, Philos. Mag. **83**, 377 (2003).

[16] I. V. Belova and G. E. Murch, Philos. Mag. **83**, 393 (2003).

[17] M. Athénes, G. Adjanors, and J. Creuze, Physical Review Materials **6**, 10.1103/physrevmaterials.6.013805 (2022).

[18] M. Nastar, V. Y. Dobretsov, and G. Martin, Philos. Mag. A **80**, 155 (2000).

[19] M. Nastar, Philosophical Magazine **85**, 3767 (2005).

[20] T. Schuler, L. Messina, and M. Nastar, Computational Materials Science **172**, 109191 (2020).

[21] K. D. Belashchenko and V. G. Vaks, J. Phys. CM **10**, 1965 (1998).

[22] V. G. Vaks, A. Y. Stroev, I. R. Pankratov, and A. D. Zabolotskiy, J. Exp. Theo. Phys. **119**, 272 (2014).

[23] V. G. Vaks, K. Y. Khromov, I. R. Pankratov, and V. V. Popov, J. Exp. Theo. Phys. **123**, 59 (2016).

[24] R. Kikuchi, Prog. Theor. Phys. Suppl. **35**, 1 (1966).

[25] H. Sato and R. Kikuchi, Phys. Rev. B **28**, 648 (1983).

[26] H. Sato, T. Ishikawa, and R. Kikuchi, J. Phys. Chem. Solids **46**, 1361 (1985).

[27] E. W. Montroll and G. H. Weiss, J. Math. Phys. **6**, 167 (1965).

[28] M. Koiwa and S. Ishioka, Philos. Mag. A **47**, 927 (1983).

[29] D. R. Trinkle, Philos. Mag. **97**, 2514 (2017).

[30] Z. W. Gortel and M. A. Załuska-Kotur, Phys. Rev. B **70**, 125431 (2004).

[31] M. A. Załuska-Kotur and Z. W. Gortel, Phys. Rev. B **76**, 245401 (2007).

[32] M. A. Załuska-Kotur, Appl. Surf. Sci. **304**, 122 (2014).

[33] D. R. Trinkle, Phys. Rev. Lett. **121**, 235901 (2018).

[34] T. Cohen and M. Welling, in *Proceedings of The 33rd International Conference on Machine Learning*, Proceedings of Machine Learning Research, Vol. 48, edited by M. F. Balcan and K. Q. Weinberger (PMLR, New York, New York, USA, 2016) pp. 2990–2999.

[35] B. Cantor, I. T. H. Chang, P. Knight, and A. J. B. Vincent, Mater. Sci. Eng. A **375-377**, 213 (2004).

[36] Z. Zhang, D. E. Armstrong, and P. S. Grant, Progress in Materials Science **123**, 100807 (2022).

[37] D. S. Gaunt and M. F. Sykes, J. Phys. A **16**, 783 (1983).

[38] H. Ouyang and B. Fultz, Journal of Applied Physics **66**, 4752 (1989).

[39] A. Gali and E. George, Intermetallics **39**, 74 (2013).

[40] Y. Wu, Y. Cai, T. Wang, J. Si, J. Zhu, Y. Wang, and X. Hui, Materials Letters **130**, 277 (2014).

[41] J. He, H. Wang, H. Huang, X. Xu, M. Chen, Y. Wu, X. Liu, T. Nieh, K. An, and Z. Lu, Acta Materialia **102**, 187 (2016).

[42] Y. Ye, Q. Wang, J. Lu, C. Liu, and Y. Yang, Materials Today **19**, 349 (2016).

[43] D. Wei, X. Li, W. Heng, Y. Koizumi, F. He, W.-M. Choi, B.-J. Lee, H. S. Kim, H. Kato, and A. Chiba, Materials Research Letters **7**, 82 (2018).

[44] W. Li, P. K. Liaw, and Y. Gao, Intermetallics **99**, 69 (2018).

[45] X. Fan, R. Qu, and Z. Zhang, Journal of Materials Science & Technology **123**, 70 (2022).

[46] K.-Y. Tsai, M.-H. Tsai, and J.-W. Yeh, Acta Materialia **61**, 4887 (2013).

[47] W.-M. Choi, Y. H. Jo, S. S. Sohn, S. Lee, and B.-J. Lee, npj Computational Materials **4**, 10.1038/s41524-017-0060-9 (2018).

[48] S. L. Thomas and S. Patala, Acta Materialia **196**, 144 (2020).

[49] J. Kottke, D. Utt, M. Laurent-Brocq, A. Fareed, D. Gaertner, L. Perrière, Ł. Rogal, A. Stukowski, K. Albe, S. V. Divinski, and G. Wilde, Acta Materialia **194**, 236 (2020).

[50] B. Xu, J. Zhang, S. Ma, Y. Xiong, S. Huang, J. Kai, and S. Zhao, Acta Materialia **234**, 118051 (2022).

[51] E. Grushka, Analytical Chemistry **44**, 1733 (1972).

[52] J. Olivier and M. Norberg, International Journal of Psychological Research **3** (2010).

[53] S. Ali, J. Ara, and I. Shah, Afrika Matematika **33**, 10.1007/s13370-022-00995-w (2022).

[54] M. Vaidya, K. Pradeep, B. Murty, G. Wilde, and S. Divinski, Acta Materialia **146**, 211 (2018).

[55] D. Gaertner, J. Kottke, Y. Chumlyakov, F. Hergemöller, G. Wilde, and S. V. Divinski, Scripta Materialia **187**, 57 (2020).

[56] D. R. Trinkle, Physical Review Letters **121**, 10.1103/physrevlett.121.235901 (2018).

[57] D. R. Trinkle, Philosophical Magazine **97**, 2514 (2017).

[58] X. Glorot, A. Bordes, and Y. Bengio, in *Proceedings of the Fourteenth International Conference on Artificial Intelligence and Statistics*, Proceedings of Machine Learning Research, Vol. 15, edited by G. Gordon, D. Dunson, and M. Dudík (PMLR, Fort Lauderdale, FL, USA, 2011) pp. 315–323.

[59] A. Paszke, S. Gross, F. Massa, A. Lerer, J. Bradbury, G. Chanan, T. Killeen, Z. Lin, N. Gimelshein, L. Antiga, A. Desmaison, A. Kopf, E. Yang, Z. DeVito, M. Raison, A. Tejani, S. Chilamkurthy, B. Steiner, L. Fang, J. Bai, and S. Chintala, in *Advances in Neural Information Processing Systems 32* (Curran Associates, Inc., 2019) pp. 8024–8035.

[60] D. P. Kingma and J. Ba, Adam: A method for stochastic optimization (2014).

[61] K. Ebihara, T. Suzudo, and M. Yamaguchi, Materials Transactions **58**, 26 (2017).

[62] A. R. Allnatt, T. R. Paul, I. V. Belova, and G. E. Murch, Philosophical Magazine **96**, 2969 (2016).

[63] J. R. Manning, Physical Review B **4**, 1111 (1971).

[64] L. K. Moleko, A. R. Allnatt, and E. L. Allnatt, Philosophical Magazine A **59**, 141 (1989).

[65] D. Frenkel and B. Smit, *Understanding molecular simulation: from algorithms to applications* (Elsevier, 2023).

[66] A. P. Thompson, H. M. Aktulga, R. Berger, D. S. Bolintineanu, W. M. Brown, P. S. Crozier, P. J. in 't Veld, A. Kohlmeyer, S. G. Moore, T. D. Nguyen, R. Shan, M. J. Stevens, J. Tranchida, C. Trott, and S. J. Plimpton, Computer Physics Communications **271**, 108171 (2022).

[67] M. N. Nounou and B. R. Bakshi, in *Data Handling in Science and Technology* (Elsevier, 2000) pp. 119–150.

[68] G. Henkelman and H. Jónsson, The Journal of Chemical Physics **113**, 9978 (2000).

[69] W. E, W. Ren, and E. Vanden-Eijnden, Physical Review B **66**, 10.1103/physrevb.66.052301 (2002).

[70] E. Maras, O. Trushin, A. Stukowski, T. Ala-Nissila, and H. Jónsson, Computer Physics Communica-

tions **205**, 13 (2016).

[71] S. E. Restrepo and P. Andric, Computational Materials Science **218**, 111978 (2023).

[72] J. Guénolé, W. G. Nöhring, A. Vaid, F. Houllé, Z. Xie, A. Prakash, and E. Bitzek, Computational Materials Science **175**, 109584 (2020).

[73] T. Garnier, V. R. Manga, D. R. Trinkle, M. Nastar, and P. Bellon, Physical Review B **88**, 10.1103/physrevb.88.134108 (2013).

[74] D. A. Porter, K. E. Easterling, and M. Y. Sherif, in *Phase Transformations in Metals and Alloys* (CRC Press, 2021).

[75] K. Sugita, N. Matsuoka, M. Mizuno, and H. Araki, Scripta Materialia **176**, 32 (2020).
